# Supplementary material for: No significant correlation between radial velocity planet presence and debris disc properties
Source: arXiv:2005.03573 ancillary file (2020-05-07)
Supplement: Supplementary file 1 [file table1.pdf]

# Full version of Table 1

| Name     | $d$ / pc | $T_{\text{eff}}$ / K | $L_{\text{star}} / L_{\odot}$ | $a_{\text{binary}}$ / au | $M \sin(i) / M_{\text{J}}$ | $a_{\text{pl}}$ / au |
|----------|----------|----------------------|-------------------------------|--------------------------|----------------------------|----------------------|
| HD 142   | 26.2     | 6200                 | 3.0E+00                       | 1.0E+02                  | 5.3E+00                    | 6.8E+00              |
| HD 1237  | 17.6     | 5460                 | 6.5E-01                       | 6.9E+01                  | 3.4E+00                    | 4.9E-01              |
| HD 1326  | 3.6      | 3444                 | 2.1E-02                       | 2.3E+01                  | 1.1E-01                    | 5.4E+00              |
| HD 1461  | 23.5     | 5736                 | 1.2E+00                       |                          | 2.0E-02                    | 6.3E-02              |
| HD 3651  | 11.1     | 5240                 | 5.3E-01                       |                          | 2.3E-01                    | 3.0E-01              |
| HD 4203  | 81.6     | 5577                 | 2.0E+00                       |                          | 2.2E+00                    | 1.2E+00              |
| HD 4208  | 34.2     | 5708                 | 8.0E-01                       |                          | 8.1E-01                    | 1.7E+00              |
| HD 4308  | 22.0     | 5676                 | 1.0E+00                       |                          | 5.0E-02                    | 1.2E-01              |
| HD 6434  | 42.4     | 5789                 | 1.3E+00                       |                          | 4.9E-01                    | 1.4E-01              |
| HD 7924  | 16.8     | 5238                 | 3.9E-01                       |                          | 2.5E-02                    | 1.1E-01              |
| HD 8574  | 44.2     | 5917                 | 2.3E+00                       |                          | 2.0E+00                    | 7.6E-01              |
| HD 8673  | 37.9     | 6392                 | 3.4E+00                       | 1.1E+01                  | 1.4E+01                    | 3.0E+00              |
| HD 9826  | 13.4     | 6258                 | 3.4E+00                       | 7.4E+02                  | 4.1E+00                    | 2.5E+00              |
| HD 10647 | 17.3     | 6101                 | 1.6E+00                       |                          | 9.4E-01                    | 2.0E+00              |
| HD 10697 | 32.6     | 5614                 | 3.0E+00                       | 3.0E+02                  | 6.4E+00                    | 2.1E+00              |
| HD 10700 | 3.6      | 5418                 | 4.8E-01                       | 4.9E+02                  | 1.2E-02                    | 1.3E+00              |
| HD 11964 | 33.6     | 5332                 | 2.9E+00                       | 1.0E+03                  | 6.2E-01                    | 3.2E+00              |
| HD 12661 | 37.9     | 5737                 | 1.3E+00                       |                          | 2.4E+00                    | 8.4E-01              |
| HD 13445 | 10.8     | 5189                 | 4.1E-01                       | 2.2E+01                  | 4.4E+00                    | 1.1E-01              |
| HD 16141 | 37.8     | 5733                 | 2.3E+00                       | 2.3E+02                  | 2.6E-01                    | 3.6E-01              |
| HD 16175 | 60.0     | 5930                 | 3.7E+00                       |                          | 5.1E+00                    | 2.1E+00              |
| HD 16417 | 25.4     | 5856                 | 2.8E+00                       | 1.1E+03                  | 7.0E-02                    | 1.4E-01              |
| HD 17051 | 17.3     | 6214                 | 1.7E+00                       |                          | 2.3E+00                    | 9.2E-01              |
| HD 20782 | 35.5     | 5779                 | 1.3E+00                       | 9.0E+03                  | 1.5E+00                    | 1.4E+00              |
| HD 20794 | 6.0      | 5441                 | 6.6E-01                       |                          | 1.5E-02                    | 5.1E-01              |
| HD 21411 | 29.2     | 5498                 | 5.5E-01                       | 5.9E+02                  | 2.1E-01                    | 3.6E-01              |
| HD 22049 | 3.2      | 5076                 | 3.3E-01                       |                          | 1.6E+00                    | 3.4E+00              |
| HD 23079 | 33.5     | 5988                 | 1.4E+00                       |                          | 2.6E+00                    | 1.6E+00              |
| HD 23127 | 94.1     | 5833                 | 2.8E+00                       |                          | 1.5E+00                    | 2.4E+00              |
| HD 23596 | 52.0     | 6067                 | 2.9E+00                       | 3.7E+03                  | 9.0E+00                    | 2.8E+00              |
| HD 26965 | 5.0      | 5191                 | 4.2E-01                       | 4.0E+02                  | 2.7E-02                    |                      |
| HD 27894 | 43.9     | 4908                 | 3.8E-01                       |                          | 5.4E+00                    | 5.5E+00              |
| HD 28185 | 39.6     | 5652                 | 1.0E+00                       | 4.0E+04                  | 5.9E+00                    | 1.0E+00              |
| HD 30177 | 55.7     | 5551                 | 1.2E+00                       |                          | 8.6E+00                    | 3.7E+00              |
| HD 30562 | 26.2     | 5951                 | 2.9E+00                       |                          | 1.2E+00                    | 2.3E+00              |
| HD 33283 | 90.1     | 5950                 | 4.1E+00                       | 5.0E+03                  | 3.3E-01                    | 1.5E-01              |
| HD 33564 | 21.0     | 6405                 | 3.3E+00                       | 7.1E+02                  | 9.1E+00                    | 1.1E+00              |
| HD 33793 | 3.9      | 3574                 | 1.2E-02                       |                          | 2.2E-02                    | 3.1E-01              |
| HD 34445 | 46.2     | 5824                 | 2.1E+00                       |                          | 8.2E-01                    | 2.1E+00              |
| HD 37124 | 31.7     | 5543                 | 7.9E-01                       | 9.5E+01                  | 7.0E-01                    | 2.8E+00              |
| HD 37605 | 46.9     | 5385                 | 7.0E-01                       |                          | 3.2E+00                    | 3.7E+00              |
| HD 38529 | 42.4     | 5582                 | 6.9E+00                       | 1.2E+04                  | 1.3E+01                    | 3.6E+00              |
| HD 39091 | 18.3     | 5970                 | 1.5E+00                       |                          | 1.0E+01                    | 3.1E+00              |
| HD 39855 | 23.3     | 5478                 | 4.9E-01                       | 2.3E+02                  | 2.7E-02                    | 4.1E-02              |
| HD 40307 | 12.9     | 4810                 | 2.5E-01                       |                          | 3.0E-02                    | 1.3E-01              |
| HD 40979 | 33.3     | 6112                 | 1.9E+00                       | 6.4E+03                  | 4.7E+00                    | 8.5E-01              |
| HD 41004 | 43.0     | 4851                 | 6.2E-01                       | 1.7E+01                  | 2.5E+00                    |                      |
| HD 42581 | 5.8      | 3398                 | 3.8E-02                       | 4.2E+01                  | 1.0E-01                    | 9.7E-01              |

| Name      | $d$ / pc | $T_{\text{eff}}$ / K | $L_{\text{star}} / L_{\odot}$ | $a_{\text{binary}}$ / au | $M \sin(i) / M_{\text{J}}$ | $a_{\text{pl}}$ / au |
|-----------|----------|----------------------|-------------------------------|--------------------------|----------------------------|----------------------|
| HD 45184  | 21.9     | 5840                 | 1.2E+00                       |                          | 3.8E-02                    | 6.4E-02              |
| HD 45350  | 46.9     | 5649                 | 1.4E+00                       |                          | 1.8E+00                    | 1.9E+00              |
| HD 49674  | 43.1     | 5608                 | 9.5E-01                       | 1.7E+04                  | 1.0E-01                    | 6.0E-02              |
| HD 50499  | 46.4     | 6041                 | 2.3E+00                       |                          | 2.9E+00                    | 9.0E+00              |
| HD 50554  | 31.2     | 5999                 | 1.5E+00                       |                          | 5.0E+00                    | 2.4E+00              |
| HD 52265  | 30.0     | 6123                 | 2.3E+00                       |                          | 1.2E+00                    | 5.2E-01              |
| HD 60532  | 25.3     | 6119                 | 9.4E+00                       | 9.1E+01                  | 2.5E+00                    | 1.6E+00              |
| HD 63454  | 37.7     | 4855                 | 2.9E-01                       |                          | 2.5E-01                    | 4.0E-02              |
| HD 65216  | 35.2     | 5622                 | 7.1E-01                       | 2.5E+02                  | 2.0E+00                    | 5.8E+00              |
| HD 66428  | 53.4     | 5673                 | 1.2E+00                       |                          | 3.2E+00                    | 3.5E+00              |
| HD 68988  | 61.0     | 5878                 | 1.6E+00                       |                          | 2.0E+00                    | 7.0E-02              |
| HD 69830  | 12.6     | 5414                 | 6.1E-01                       | 8.7E+01                  | 5.7E-02                    | 6.3E-01              |
| HD 70573  | 45.7     | 5763                 | 1.0E+00                       | 1.6E+02                  | 6.1E+00                    | 1.8E+00              |
| HD 72659  | 51.4     | 5857                 | 2.4E+00                       |                          | 3.9E+00                    | 4.8E+00              |
| HD 73526  | 97.5     | 5620                 | 2.1E+00                       |                          | 3.1E+00                    | 6.5E-01              |
| HD 74156  | 64.6     | 5946                 | 2.5E+00                       |                          | 8.1E+00                    | 3.9E+00              |
| HD 75289  | 29.1     | 6153                 | 2.0E+00                       | 6.3E+02                  | 4.9E-01                    | 5.0E-02              |
| HD 75732  | 12.6     | 5334                 | 6.3E-01                       | 1.1E+03                  | 3.9E+00                    | 5.5E+00              |
| HD 76700  | 61.0     | 5677                 | 1.8E+00                       | 3.4E+02                  | 2.1E-01                    | 5.0E-02              |
| HD 80606  | 66.6     | 5498                 | 9.8E-01                       | 1.4E+03                  | 4.4E+00                    |                      |
| HD 81040  | 34.5     | 5728                 | 8.4E-01                       |                          | 7.3E+00                    | 1.9E+00              |
| HD 82943  | 27.6     | 6040                 | 1.5E+00                       |                          | 2.0E+00                    | 7.4E-01              |
| HD 83443  | 41.0     | 5468                 | 8.1E-01                       | 4.7E+02                  | 3.4E-01                    | 4.0E-02              |
| HD 85512  | 11.3     | 4337                 | 1.7E-01                       |                          | 1.0E-02                    | 2.6E-01              |
| HD 87883  | 18.3     | 5005                 | 3.4E-01                       |                          | 1.5E+00                    | 3.6E+00              |
| HD 88133  | 73.8     | 5428                 | 3.2E+00                       |                          | 2.9E-01                    | 4.8E-02              |
| HD 89307  | 32.0     | 5931                 | 1.4E+00                       |                          | 2.1E+00                    | 3.3E+00              |
| HD 89744  | 39.0     | 6212                 | 6.3E+00                       | 2.2E+02                  | 8.4E+00                    | 9.2E-01              |
| HD 90156  | 22.0     | 5598                 | 7.3E-01                       |                          | 5.7E-02                    | 2.5E-01              |
| HD 92788  | 34.7     | 5823                 | 1.2E+00                       |                          | 3.8E+00                    | 9.7E-01              |
| HD 93083  | 28.5     | 5022                 | 4.0E-01                       |                          | 3.7E-01                    | 4.8E-01              |
| HD 95128  | 13.8     | 5981                 | 1.5E+00                       |                          | 2.5E+00                    | 2.1E+00              |
| HD 95735  | 2.6      | 3446                 | 2.0E-02                       |                          | 9.4E-03                    | 7.9E-02              |
| HD 97658  | 21.6     | 5181                 | 3.6E-01                       |                          | 3.0E-02                    |                      |
| HD 99492  | 55.7     | 4948                 | 3.5E-01                       | 1.6E+03                  | 7.0E-02                    | 1.2E-01              |
| HD 101930 | 30.1     | 5154                 | 4.7E-01                       | 2.2E+03                  | 2.5E-01                    | 3.0E-01              |
| HD 102117 | 39.6     | 5650                 | 1.4E+00                       |                          | 1.7E-01                    | 1.5E-01              |
| HD 102195 | 29.4     | 5321                 | 4.9E-01                       | 3.5E+02                  | 4.1E-01                    | 5.0E-02              |
| HD 102365 | 9.3      | 5671                 | 8.5E-01                       | 2.1E+02                  | 5.0E-02                    | 4.6E-01              |
| HD 104067 | 20.4     | 4919                 | 3.1E-01                       |                          | 1.6E-01                    | 2.6E-01              |
| HD 106252 | 37.4     | 5855                 | 1.4E+00                       |                          | 6.9E+00                    | 2.6E+00              |
| HD 107148 | 49.5     | 5772                 | 1.3E+00                       | 1.7E+03                  | 2.1E-01                    | 2.7E-01              |
| HD 108147 | 39.0     | 6255                 | 2.0E+00                       | 1.1E+02                  | 2.6E-01                    | 1.0E-01              |
| HD 108874 | 68.5     | 5508                 | 9.9E-01                       |                          | 1.4E+00                    | 1.0E+00              |
| HD 109749 | 63.2     | 5780                 | 1.8E+00                       | 5.6E+02                  | 2.7E-01                    | 6.2E-02              |
| HD 111232 | 29.0     | 5502                 | 7.0E-01                       |                          | 7.1E+00                    | 2.0E+00              |
| HD 113337 | 36.2     | 6689                 | 4.1E+00                       | 1.8E+02                  | 2.8E+00                    | 9.2E-01              |
| HD 113538 | 15.9     | 4060                 | 1.3E-01                       |                          | 9.3E-01                    | 2.4E+00              |
| HD 114386 | 28.0     | 4871                 | 3.0E-01                       |                          | 1.1E+00                    | 1.7E+00              |
| HD 114613 | 20.3     | 5676                 | 4.2E+00                       |                          | 3.6E-01                    | 5.3E+00              |
| HD 114729 | 37.9     | 5822                 | 2.6E+00                       | 3.1E+02                  | 8.3E-01                    | 2.1E+00              |
| HD 114762 | 40.2     | 5909                 | 1.7E+00                       | 1.3E+02                  | 1.1E+01                    | 3.6E-01              |
| HD 114783 | 20.4     | 5048                 | 4.1E-01                       |                          | 1.1E+00                    | 1.2E+00              |
| HD 115617 | 8.5      | 5566                 | 8.3E-01                       | 1.9E+03                  | 7.2E-02                    | 4.8E-01              |
| HD 117176 | 17.9     | 5473                 | 3.0E+00                       | 5.2E+01                  | 7.4E+00                    | 4.8E-01              |
| HD 117207 | 32.4     | 5655                 | 1.2E+00                       |                          | 1.9E+00                    | 3.8E+00              |
| HD 117618 | 37.8     | 5974                 | 1.6E+00                       |                          | 1.7E-01                    | 1.8E-01              |

| Name       | $d$ / pc | $T_{\text{eff}}$ / K | $L_{\text{star}} / L_{\odot}$ | $a_{\text{binary}}$ / au | $M \sin(i) / M_{\text{J}}$ | $a_{\text{pl}}$ / au |
|------------|----------|----------------------|-------------------------------|--------------------------|----------------------------|----------------------|
| HD 118203  | 92.5     | 5784                 | 4.6E+00                       |                          | 2.8E+00                    | 7.0E-02              |
| HD 120136  | 15.7     | 6390                 | 3.1E+00                       | 1.9E+02                  | 4.3E+00                    | 4.9E-02              |
| HD 121504  | 41.7     | 5969                 | 1.4E+00                       | 1.3E+02                  | 1.5E+00                    | 3.3E-01              |
| HD 128311  | 16.5     | 4843                 | 2.9E-01                       | 1.6E+02                  | 3.8E+00                    | 1.7E+00              |
| HD 130322  | 31.9     | 5369                 | 5.7E-01                       | 2.4E+02                  | 1.2E+00                    | 9.3E-02              |
| HD 134987  | 22.2     | 5844                 | 1.5E+00                       |                          | 1.6E+00                    | 8.1E-01              |
| HD 136352  | 14.8     | 5733                 | 1.0E+00                       |                          | 3.4E-02                    | 1.7E-01              |
| HD 141937  | 33.4     | 5869                 | 1.2E+00                       |                          | 9.7E+00                    | 1.5E+00              |
| HD 142022  | 34.3     | 5490                 | 8.8E-01                       | 6.5E+02                  | 4.4E+00                    | 2.9E+00              |
| HD 142415  | 35.6     | 5911                 | 1.3E+00                       | 5.7E+01                  | 1.7E+00                    | 1.1E+00              |
| HD 143105  | 48.7     | 6261                 | 3.6E+00                       |                          | 1.2E+00                    | 3.8E-02              |
| HD 143761  | 17.2     | 5827                 | 1.8E+00                       | 2.0E+03                  | 1.0E+00                    | 2.2E-01              |
| HD 145675  | 17.9     | 5350                 | 6.9E-01                       | 7.7E+01                  | 4.7E+00                    | 2.9E+00              |
| HD 147379  | 10.8     | 4048                 | 9.6E-02                       | 6.9E+02                  | 9.0E-02                    | 3.2E-01              |
| HD 147513  | 12.9     | 5876                 | 1.0E+00                       | 4.5E+03                  | 1.2E+00                    | 1.3E+00              |
| HD 149026  | 76.0     | 6087                 | 2.6E+00                       |                          | 3.8E-01                    |                      |
| HD 149143  | 73.4     | 5857                 | 3.2E+00                       |                          | 1.3E+00                    | 5.3E-02              |
| HD 150706  | 28.3     | 5923                 | 1.1E+00                       |                          | 2.7E+00                    | 6.7E+00              |
| HD 154345  | 18.3     | 5486                 | 6.0E-01                       |                          | 8.2E-01                    | 4.2E+00              |
| HD 154857  | 63.6     | 5499                 | 4.7E+00                       |                          | 2.6E+00                    | 5.4E+00              |
| HD 155358  | 43.0     | 5915                 | 2.1E+00                       |                          | 9.9E-01                    | 6.3E-01              |
| HD 156668  | 24.4     | 4818                 | 2.9E-01                       |                          | 1.3E-02                    | 5.0E-02              |
| HD 156846  | 47.8     | 5979                 | 4.8E+00                       | 6.2E+01                  | 1.1E+01                    | 1.1E+00              |
| HD 159868  | 55.9     | 5483                 | 3.6E+00                       | 2.0E+02                  | 2.2E+00                    | 2.3E+00              |
| HD 160691  | 15.6     | 5847                 | 1.9E+00                       |                          | 1.8E+00                    | 5.2E+00              |
| HD 162004  | 22.2     | 6226                 | 2.1E+00                       | 6.9E+02                  | 1.5E+00                    | 4.4E+00              |
| HD 162020  | 30.9     | 4574                 | 2.7E-01                       | 4.2E+01                  | 9.8E+00                    | 8.0E-02              |
| HD 164922  | 22.1     | 5358                 | 7.2E-01                       | 1.3E+03                  | 3.1E-01                    | 2.1E+00              |
| HD 168443  | 39.7     | 5567                 | 2.4E+00                       | 4.8E+01                  | 1.7E+01                    | 2.8E+00              |
| HD 168746  | 41.6     | 5565                 | 1.0E+00                       | 1.4E+02                  | 2.7E-01                    | 7.0E-02              |
| HD 169830  | 37.6     | 6274                 | 5.0E+00                       | 4.2E+02                  | 4.0E+00                    | 3.6E+00              |
| HD 177565  | 16.9     | 5641                 | 8.7E-01                       |                          | 4.8E-02                    | 2.5E-01              |
| HD 178911B | 47.0     | 5328                 | 1.2E+00                       | 7.8E+02                  | 8.0E+00                    | 3.4E-01              |
| HD 179949  | 27.5     | 6205                 | 2.0E+00                       | 4.0E+02                  | 9.2E-01                    | 4.4E-02              |
| HD 180617  | 5.9      | 3396                 | 3.2E-02                       | 2.8E+01                  | 3.8E-02                    | 3.4E-01              |
| HD 183263  | 54.3     | 5931                 | 1.8E+00                       | 1.8E+02                  | 4.0E+00                    | 1.5E+00              |
| HD 185269  | 52.1     | 5885                 | 5.0E+00                       | 2.3E+02                  | 1.0E+00                    | 7.7E-02              |
| HD 186427  | 21.4     | 5791                 | 1.3E+00                       | 8.2E+02                  | 1.8E+00                    | 1.7E+00              |
| HD 187085  | 46.0     | 6098                 | 2.3E+00                       |                          | 8.4E-01                    | 2.1E+00              |
| HD 187123  | 46.0     | 5781                 | 1.3E+00                       | 1.2E+02                  | 2.0E+00                    | 4.9E+00              |
| HD 188015  | 50.7     | 5702                 | 1.1E+00                       | 2.1E+02                  | 1.5E+00                    | 1.2E+00              |
| HD 189733  | 19.8     | 4991                 | 3.4E-01                       | 2.3E+02                  | 1.1E+00                    |                      |
| HD 192263  | 19.7     | 4924                 | 3.1E-01                       | 1.4E+02                  | 5.6E-01                    | 1.5E-01              |
| HD 192310  | 8.8      | 5063                 | 4.0E-01                       |                          | 7.6E-02                    | 1.2E+00              |
| HD 195019  | 37.7     | 5608                 | 2.2E+00                       | 1.5E+02                  | 4.0E+00                    | 1.4E-01              |
| HD 196050  | 50.8     | 5831                 | 2.2E+00                       | 5.6E+02                  | 3.2E+00                    | 2.5E+00              |
| HD 196885  | 34.2     | 6188                 | 2.7E+00                       | 2.2E+01                  | 2.6E+00                    | 2.4E+00              |
| HD 202206  | 45.5     | 5695                 | 1.1E+00                       |                          | 1.8E+01                    | 2.4E+00              |
| HD 204961  | 5.0      | 3498                 | 2.8E-02                       |                          | 6.8E-01                    | 3.6E+00              |
| HD 208487  | 44.0     | 6183                 | 1.7E+00                       |                          | 5.2E-01                    | 5.2E-01              |
| HD 209458  | 48.4     | 6096                 | 1.7E+00                       |                          | 7.3E-01                    |                      |
| HD 210277  | 21.3     | 5640                 | 9.8E-01                       | 1.4E+02                  | 1.3E+00                    | 1.1E+00              |
| HD 211970  | 13.0     | 4108                 | 8.3E-02                       |                          | 4.1E-02                    | 1.4E-01              |
| HD 212301  | 54.3     | 5998                 | 2.0E+00                       | 2.4E+02                  | 5.1E-01                    | 3.0E-02              |
| HD 213240  | 40.9     | 5927                 | 2.7E+00                       | 8.2E+02                  | 5.6E+00                    | 1.9E+00              |
| HD 215152  | 21.6     | 4784                 | 2.9E-01                       |                          | 9.1E-03                    | 1.5E-01              |
| HD 216435  | 33.0     | 6039                 | 3.6E+00                       |                          | 1.3E+00                    | 2.6E+00              |

| Name       | $d$ / pc | $T_{\text{eff}}$ / K | $L_{\text{star}} / L_{\odot}$ | $a_{\text{binary}}$ / au | $M \sin(i) / M_{\text{J}}$ | $a_{\text{pl}}$ / au |
|------------|----------|----------------------|-------------------------------|--------------------------|----------------------------|----------------------|
| HD 216437  | 26.7     | 5908                 | 2.3E+00                       |                          | 2.2E+00                    | 2.5E+00              |
| HD 216770  | 36.7     | 5423                 | 7.0E-01                       |                          | 5.7E-01                    | 4.6E-01              |
| HD 217014  | 15.5     | 5921                 | 1.4E+00                       | 4.5E+01                  | 4.7E-01                    | 5.3E-02              |
| HD 217107  | 20.1     | 5697                 | 1.2E+00                       | 8.0E+00                  | 2.6E+00                    | 5.3E+00              |
| HD 219134  | 6.6      | 4873                 | 2.9E-01                       | 4.6E+01                  | 3.4E-01                    | 3.1E+00              |
| HD 221420  | 31.2     | 5837                 | 4.0E+00                       |                          | 9.7E+00                    | 1.9E+01              |
| HD 222582  | 42.2     | 5795                 | 1.3E+00                       | 4.7E+03                  | 8.4E+00                    | 1.3E+00              |
| HD 224693  | 93.8     | 5926                 | 3.8E+00                       |                          | 7.0E-01                    | 1.9E-01              |
| HD 285968  | 9.5      | 3460                 | 3.5E-02                       |                          | 2.6E-02                    | 6.6E-02              |
| HD 330075  | 45.4     | 4996                 | 3.9E-01                       | 1.5E+02                  | 4.8E-01                    | 4.0E-02              |
| HIP 5643   | 3.6      | 2931                 | 2.2E-03                       |                          | 3.6E-03                    | 2.8E-02              |
| HIP 12961  | 23.4     | 4111                 | 9.3E-02                       |                          | 3.6E-01                    | 2.5E-01              |
| HIP 14810  | 50.6     | 5578                 | 9.2E-01                       |                          | 3.9E+00                    | 7.0E-02              |
| HIP 19165  | 25.9     | 4369                 | 1.4E-01                       |                          | 3.2E-02                    | 5.3E-02              |
| HIP 22627  | 12.4     | 3140                 | 1.6E-02                       |                          | 8.2E-01                    | 2.4E+00              |
| HIP 36208  | 3.8      | 3141                 | 9.7E-03                       |                          | 9.1E-03                    | 9.1E-02              |
| HIP 43790  | 20.5     | 3967                 | 9.9E-02                       |                          | 2.3E+00                    | 4.5E+00              |
| HIP 56528  | 9.1      | 3502                 | 3.4E-02                       |                          | 1.4E-01                    | 3.6E+00              |
| HIP 57050  | 11.0     | 3151                 | 1.5E-02                       |                          | 3.0E-01                    | 1.7E-01              |
| HIP 57087  | 9.8      | 3437                 | 2.4E-02                       |                          | 7.0E-02                    | 2.9E-02              |
| HIP 57548  | 3.4      | 3005                 | 3.7E-03                       |                          | 4.4E-03                    | 5.0E-02              |
| HIP 70849  | 24.1     | 3993                 | 9.2E-02                       |                          | 9.0E+00                    | 2.0E+01              |
| HIP 70890  | 1.3      | 2656                 | 1.3E-03                       |                          | 4.0E-03                    | 4.9E-02              |
| HIP 74995  | 6.3      | 3225                 | 1.2E-02                       |                          | 5.0E-02                    | 4.1E-02              |
| HIP 80459  | 6.5      | 3411                 | 1.4E-02                       | 3.5E+01                  | 8.9E-03                    | 7.8E-02              |
| HIP 80824  | 4.3      | 3136                 | 1.1E-02                       | 2.2E+01                  | 2.4E-02                    | 4.7E-01              |
| HIP 83043  | 10.4     | 3598                 | 4.5E-02                       |                          | 3.3E-01                    | 1.1E+00              |
| HIP 85523  | 4.6      | 3389                 | 1.6E-02                       |                          | 3.5E-02                    | 3.9E-02              |
| HIP 85647  | 16.9     | 3862                 | 9.3E-02                       | 8.3E+02                  | 6.8E+00                    | 6.6E+00              |
| HIP 86162  | 4.6      | 3502                 | 2.2E-02                       |                          | 6.0E-02                    | 1.7E-01              |
| HIP 86214  | 5.0      | 3055                 | 8.0E-03                       |                          | 2.7E-02                    | 1.8E-01              |
| HIP 86287  | 8.2      | 3547                 | 3.0E-02                       |                          | 2.1E-02                    | 9.2E-02              |
| HIP 109388 | 8.8      | 3327                 | 2.8E-02                       |                          | 1.0E+00                    | 2.4E+00              |
| HIP 113020 | 4.7      | 3129                 | 1.3E-02                       |                          | 2.3E+00                    | 2.1E-01              |
| GJ 317     | 15.1     | 3225                 | 2.3E-02                       |                          | 2.5E+00                    | 1.2E+00              |
| GJ 1214    | 14.6     | 3053                 | 3.6E-03                       |                          | 2.0E-02                    | 1.4E-02              |
| GJ 3323    | 5.3      | 3005                 | 3.5E-03                       |                          | 7.3E-03                    | 1.3E-01              |
| GJ 3634    | 19.8     | 3429                 | 2.9E-02                       |                          | 2.6E-02                    | 2.9E-02              |
| BD-10 3166 | 80.0     | 5312                 | 6.5E-01                       | 1.6E+03                  | 5.9E-01                    | 4.0E-02              |
