# Supplementary material for: No significant correlation between radial velocity planet presence and debris disc properties
Source: arXiv:2005.03573 ancillary file (2020-05-07)
Supplement: Supplementary file 2 [file table2.pdf]

# Full version of Table 2

| Name     | $d$ / pc | $T_{\text{eff}}$ / K | $L/L_{\odot}$ | $a_{\text{binary}}$ / au |
|----------|----------|----------------------|---------------|--------------------------|
| HD 166   | 13.7     | 5513                 | 6.3E-01       |                          |
| HD 693   | 18.7     | 6196                 | 3.0E+00       |                          |
| HD 739   | 21.3     | 6481                 | 3.0E+00       |                          |
| HD 1581  | 8.6      | 5965                 | 1.3E+00       |                          |
| HD 1835  | 20.9     | 5841                 | 1.1E+00       |                          |
| HD 3443  | 15.4     | 5449                 | 1.2E+00       | 8.9E+00                  |
| HD 4391  | 15.2     | 5781                 | 9.6E-01       | 2.5E+02                  |
| HD 4628  | 7.4      | 4993                 | 2.9E-01       |                          |
| HD 4676  | 23.5     | 6232                 | 4.3E+00       | 1.3E-01                  |
| HD 4747  | 18.7     | 5364                 | 4.5E-01       | 7.2E+00                  |
| HD 4813  | 15.8     | 6250                 | 1.8E+00       |                          |
| HD 4967  | 15.6     | 4250                 | 1.1E-01       | 2.6E+02                  |
| HD 5133  | 14.2     | 4878                 | 2.8E-01       |                          |
| HD 7439  | 23.4     | 6444                 | 4.1E+00       | 1.2E+03                  |
| HD 7570  | 15.1     | 6233                 | 2.0E+00       |                          |
| HD 9540  | 19       | 5427                 | 5.5E-01       |                          |
| HD 10307 | 12.7     | 5885                 | 1.5E+00       | 7.4E+00                  |
| HD 10361 | 7.7      | 4596                 | 2.2E-01       | 8.6E+01                  |
| HD 10476 | 7.5      | 5232                 | 4.4E-01       | 6.9E-01                  |
| HD 11507 | 11       | 3921                 | 8.1E-02       |                          |
| HD 13974 | 10.8     | 5687                 | 1.2E+00       | 9.6E-02                  |
| HD 14412 | 12.7     | 5428                 | 4.4E-01       |                          |
| HD 16160 | 7.2      | 4828                 | 2.8E-01       | 1.5E+01                  |
| HD 16673 | 21.8     | 6231                 | 1.9E+00       |                          |
| HD 16765 | 22.7     | 6161                 | 2.1E+00       | 9.1E+01                  |
| HD 17206 | 14.2     | 6415                 | 2.7E+00       |                          |
| HD 17925 | 10.3     | 5143                 | 4.0E-01       | 7.0E-02                  |
| HD 19305 | 14.7     | 4096                 | 1.0E-01       |                          |
| HD 20010 | 14.2     | 6118                 | 4.6E+00       | 5.5E+01                  |
| HD 20630 | 9.1      | 5718                 | 8.4E-01       |                          |
| HD 20807 | 12       | 5903                 | 1.0E+00       | 3.7E+03                  |
| HD 21197 | 15.4     | 4546                 | 2.2E-01       |                          |
| HD 21531 | 12.5     | 3989                 | 1.2E-01       |                          |
| HD 22484 | 14       | 5991                 | 3.2E+00       |                          |
| HD 22496 | 13.6     | 4202                 | 1.2E-01       |                          |
| HD 23356 | 14       | 4984                 | 3.0E-01       |                          |
| HD 23754 | 17.6     | 6585                 | 5.1E+00       |                          |
| HD 27274 | 13       | 4475                 | 1.9E-01       |                          |
| HD 30495 | 13.3     | 5836                 | 9.6E-01       |                          |
| HD 30652 | 8.1      | 6423                 | 2.8E+00       |                          |
| HD 32147 | 8.7      | 4803                 | 3.0E-01       |                          |
| HD 33262 | 11.6     | 6202                 | 1.5E+00       | 3.7E+03                  |
| HD 36435 | 19.2     | 5459                 | 5.5E-01       |                          |
| HD 36705 | 15.2     | 4910                 | 4.1E-01       | 3.1E+00                  |
| HD 38393 | 8.9      | 6363                 | 2.4E+00       | 8.6E+02                  |
| HD 43162 | 16.7     | 5588                 | 7.0E-01       | 4.1E+02                  |
| HD 43834 | 10.2     | 5612                 | 8.6E-01       | 3.1E+01                  |
| HD 46588 | 17.9     | 6217                 | 1.8E+00       |                          |

| Name      | $d$ / pc | $T_{\text{eff}}$ / K | $L/L_{\odot}$ | $a_{\text{binary}}$ / au |
|-----------|----------|----------------------|---------------|--------------------------|
| HD 48682  | 16.7     | 6040                 | 1.8E+00       |                          |
| HD 50692  | 17.2     | 5925                 | 1.3E+00       |                          |
| HD 52711  | 19.2     | 5878                 | 1.3E+00       |                          |
| HD 53705  | 16.9     | 5823                 | 1.5E+00       | 3.6E+02                  |
| HD 55575  | 16.9     | 5894                 | 1.5E+00       |                          |
| HD 58855  | 20.2     | 6346                 | 2.5E+00       |                          |
| HD 61606  | 14.2     | 4831                 | 2.8E-01       | 8.3E+02                  |
| HD 62613  | 17.2     | 5551                 | 6.3E-01       |                          |
| HD 68146  | 22.4     | 6338                 | 2.6E+00       | 2.1E+03                  |
| HD 69897  | 18.3     | 6239                 | 2.4E+00       |                          |
| HD 71243  | 19.6     | 6631                 | 7.1E+00       |                          |
| HD 72905  | 14.4     | 5853                 | 1.0E+00       |                          |
| HD 76151  | 17.4     | 5826                 | 9.7E-01       |                          |
| HD 76932  | 21       | 5948                 | 1.9E+00       |                          |
| HD 76943  | 16.1     | 6614                 | 4.3E+00       | 4.6E+02                  |
| HD 78154  | 20.4     | 6210                 | 4.4E+00       | 7.3E+01                  |
| HD 78366  | 19.2     | 5938                 | 1.3E+00       |                          |
| HD 79028  | 19.6     | 5877                 | 2.8E+00       | 1.4E-01                  |
| HD 79096  | 20.4     | 5384                 | 9.8E-01       | 2.4E+00                  |
| HD 79210  | 6.1      | 3691                 | 6.0E-02       | 1.1E+02                  |
| HD 81997  | 17.3     | 6497                 | 3.7E+00       | 4.4E+00                  |
| HD 82106  | 12.9     | 5016                 | 2.3E-01       |                          |
| HD 82328  | 13.5     | 6253                 | 8.6E+00       | 5.5E+01                  |
| HD 84117  | 15       | 6189                 | 1.9E+00       |                          |
| HD 84737  | 18.3     | 5933                 | 2.8E+00       |                          |
| HD 86728  | 15.1     | 5800                 | 1.4E+00       |                          |
| HD 88230  | 4.9      | 4055                 | 1.1E-01       |                          |
| HD 89125  | 22.8     | 6088                 | 2.1E+00       | 1.7E+02                  |
| HD 89269  | 20.2     | 5652                 | 7.9E-01       |                          |
| HD 89449  | 21.4     | 6510                 | 4.3E+00       |                          |
| HD 90089  | 21.5     | 6674                 | 3.3E+00       |                          |
| HD 90839  | 12.8     | 6208                 | 1.7E+00       | 7.6E+00                  |
| HD 97101  | 12       | 3943                 | 1.2E-01       | 4.1E+02                  |
| HD 97584  | 14.6     | 4732                 | 2.2E-01       | 9.7E+01                  |
| HD 98712  | 13.2     | 3937                 | 1.2E-01       | 6.0E+01                  |
| HD 100180 | 23.3     | 6018                 | 1.4E+00       |                          |
| HD 100623 | 9.6      | 5203                 | 3.6E-01       | 1.6E+02                  |
| HD 101177 | 23.2     | 6122                 | 1.4E+00       | 2.1E+02                  |
| HD 101501 | 9.6      | 5613                 | 6.4E-01       |                          |
| HD 101581 | 12.4     | 4500                 | 1.6E-01       |                          |
| HD 102438 | 17.5     | 5601                 | 7.2E-01       |                          |
| HD 102870 | 10.9     | 6117                 | 3.7E+00       |                          |
| HD 103095 | 9.1      | 5119                 | 2.2E-01       |                          |
| HD 103932 | 10.2     | 4477                 | 2.2E-01       |                          |
| HD 106516 | 22.3     | 6267                 | 1.5E+00       | 2.0E+00                  |
| HD 108954 | 21.8     | 6056                 | 1.4E+00       |                          |
| HD 109358 | 8.4      | 5907                 | 1.3E+00       |                          |
| HD 110315 | 14.2     | 4485                 | 1.9E-01       |                          |
| HD 110833 | 14.9     | 4891                 | 3.7E-01       | 7.9E-01                  |
| HD 110897 | 17.4     | 5889                 | 1.1E+00       |                          |
| HD 111395 | 16.9     | 5616                 | 7.9E-01       |                          |
| HD 111631 | 10.6     | 3986                 | 1.0E-01       |                          |
| HD 114710 | 9.1      | 6051                 | 1.4E+00       |                          |
| HD 115404 | 11.1     | 4544                 | 2.5E-01       | 8.0E+01                  |
| HD 116442 | 15.8     | 5238                 | 4.0E-01       | 4.2E+02                  |
| HD 117043 | 21.2     | 5556                 | 9.8E-01       |                          |
| HD 118926 | 14.8     | 3944                 | 7.3E-02       |                          |

| Name      | $d$ / pc | $T_{\text{eff}}$ / K | $L/L_{\odot}$ | $a_{\text{binary}}$ / au |
|-----------|----------|----------------------|---------------|--------------------------|
| HD 119850 | 5.4      | 3580                 | 3.4E-02       |                          |
| HD 120036 | 14.6     | 4258                 | 1.1E-01       | 1.3E+02                  |
| HD 120467 | 14.3     | 4279                 | 1.6E-01       |                          |
| HD 120476 | 13.4     | 4548                 | 3.6E-01       | 4.6E+01                  |
| HD 120690 | 19.5     | 5462                 | 8.5E-01       | 2.7E+00                  |
| HD 122064 | 10.1     | 4855                 | 2.9E-01       |                          |
| HD 122742 | 17       | 5363                 | 8.4E-01       | 4.8E+00                  |
| HD 124580 | 21.2     | 5945                 | 1.1E+00       |                          |
| HD 125276 | 18.1     | 5964                 | 1.2E+00       | 5.6E+01                  |
| HD 126053 | 17.2     | 5726                 | 8.4E-01       |                          |
| HD 126660 | 14.5     | 6253                 | 4.1E+00       | 1.0E+03                  |
| HD 128165 | 13.2     | 4729                 | 2.6E-01       |                          |
| HD 128642 | 19.9     | 5240                 | 6.7E-01       | 6.3E-01                  |
| HD 129502 | 18.3     | 6657                 | 7.6E+00       |                          |
| HD 130948 | 18.2     | 6022                 | 1.2E+00       | 4.8E+01                  |
| HD 131156 | 6.7      | 4215                 | 3.6E-01       | 3.6E+01                  |
| HD 131511 | 11.5     | 5073                 | 5.1E-01       | 4.9E-01                  |
| HD 131977 | 5.9      | 3975                 | 1.4E-01       | 1.4E+02                  |
| HD 134083 | 19.6     | 6606                 | 3.2E+00       |                          |
| HD 135204 | 17.7     | 5391                 | 6.5E-01       | 1.8E+00                  |
| HD 136923 | 19.6     | 5357                 | 5.0E-01       |                          |
| HD 137763 | 19.9     | 5170                 | 6.5E-01       | 1.8E+00                  |
| HD 139763 | 15.6     | 4258                 | 1.2E-01       |                          |
| HD 140538 | 14.7     | 5616                 | 8.6E-01       | 6.2E+01                  |
| HD 141004 | 12.1     | 5990                 | 2.0E+00       |                          |
| HD 141272 | 21.3     | 5212                 | 4.8E-01       | 3.8E+02                  |
| HD 142267 | 17.3     | 5837                 | 9.7E-01       | 5.7E-01                  |
| HD 142373 | 15.9     | 5867                 | 3.2E+00       |                          |
| HD 142860 | 11.3     | 6321                 | 3.0E+00       |                          |
| HD 144579 | 14.5     | 5303                 | 4.3E-01       | 1.0E+03                  |
| HD 146361 | 21.2     | 6009                 | 3.5E+00       | 2.3E-02                  |
| HD 147584 | 12.1     | 6041                 | 1.4E+00       | 1.2E-01                  |
| HD 151288 | 9.8      | 4094                 | 1.1E-01       |                          |
| HD 153597 | 15.3     | 6184                 | 2.2E+00       | 3.0E-01                  |
| HD 154577 | 13.6     | 4863                 | 2.2E-01       |                          |
| HD 155876 | 6.4      | 3485                 | 2.8E-02       | 2.4E+00                  |
| HD 157214 | 14.3     | 5753                 | 1.3E+00       |                          |
| HD 157881 | 7.7      | 3864                 | 1.1E-01       |                          |
| HD 158633 | 12.8     | 5287                 | 4.2E-01       |                          |
| HD 160032 | 21.4     | 6612                 | 4.5E+00       |                          |
| HD 160922 | 23.2     | 6534                 | 5.4E+00       | 6.8E-02                  |
| HD 165499 | 17.6     | 6007                 | 1.7E+00       |                          |
| HD 166348 | 13.1     | 4311                 | 1.3E-01       |                          |
| HD 166620 | 11       | 5026                 | 3.5E-01       |                          |
| HD 167425 | 23       | 5997                 | 1.5E+00       | 1.8E+02                  |
| HD 168151 | 22.9     | 6440                 | 4.3E+00       | 7.7E+01                  |
| HD 170153 | 8        | 6025                 | 2.1E+00       | 4.7E+01                  |
| HD 173739 | 3.5      | 3198                 | 1.2E-02       | 4.7E+01                  |
| HD 179930 | 15.5     | 3876                 | 1.1E-01       | 3.3E+00                  |
| HD 180161 | 20       | 5440                 | 5.9E-01       |                          |
| HD 181321 | 18.8     | 5780                 | 8.8E-01       |                          |
| HD 185395 | 18.3     | 6691                 | 4.3E+00       | 7.7E+01                  |
| HD 189245 | 21.2     | 6312                 | 2.2E+00       |                          |
| HD 189567 | 17.7     | 5746                 | 1.0E+00       |                          |
| HD 190007 | 12.9     | 4496                 | 2.1E-01       |                          |
| HD 190422 | 23.4     | 6103                 | 1.5E+00       |                          |
| HD 191849 | 6.2      | 3832                 | 5.9E-02       |                          |

| Name      | $d$ / pc | $T_{\text{eff}}$ / K | $L/L_{\odot}$ | $a_{\text{binary}}$ / au |
|-----------|----------|----------------------|---------------|--------------------------|
| HD 194640 | 19.5     | 5574                 | 7.5E-01       |                          |
| HD 196761 | 14.4     | 5485                 | 5.6E-01       |                          |
| HD 196877 | 12.2     | 4088                 | 8.6E-02       |                          |
| HD 197076 | 20.9     | 5827                 | 1.0E+00       | 2.6E+03                  |
| HD 197692 | 14.7     | 6620                 | 3.6E+00       |                          |
| HD 199260 | 22       | 6281                 | 2.0E+00       |                          |
| HD 200525 | 19.8     | 5758                 | 1.9E+00       | 4.0E+00                  |
| HD 200779 | 15.1     | 4322                 | 1.7E-01       |                          |
| HD 200968 | 17.6     | 5132                 | 4.2E-01       | 7.6E+01                  |
| HD 202275 | 18.4     | 6242                 | 4.5E+00       | 3.6E+00                  |
| HD 202560 | 3.9      | 3711                 | 6.8E-02       |                          |
| HD 203244 | 20.4     | 5432                 | 6.3E-01       |                          |
| HD 203608 | 9.3      | 6133                 | 1.5E+00       |                          |
| HD 205390 | 14.6     | 4992                 | 3.1E-01       |                          |
| HD 207129 | 16       | 5956                 | 1.2E+00       | 8.8E+02                  |
| HD 209100 | 3.6      | 4654                 | 2.1E-01       | 1.5E+03                  |
| HD 210027 | 11.7     | 6444                 | 3.5E+00       | 1.0E-01                  |
| HD 210302 | 18.3     | 6428                 | 2.9E+00       |                          |
| HD 212330 | 20.6     | 5658                 | 2.8E+00       |                          |
| HD 213845 | 22.7     | 6570                 | 3.5E+00       | 1.4E+02                  |
| HD 214749 | 13.6     | 4505                 | 1.8E-01       |                          |
| HD 214953 | 23.6     | 6022                 | 1.9E+00       | 1.8E+02                  |
| HD 215648 | 16.3     | 6172                 | 4.5E+00       | 1.9E+02                  |
| HD 216133 | 14.1     | 3796                 | 6.0E-02       |                          |
| HD 216899 | 6.8      | 3702                 | 5.2E-02       |                          |
| HD 217357 | 8.2      | 4064                 | 9.3E-02       |                          |
| HD 217987 | 3.3      | 3584                 | 3.4E-02       |                          |
| HD 218511 | 15       | 4378                 | 1.6E-01       |                          |
| HD 219482 | 20.5     | 6239                 | 1.9E+00       |                          |
| HD 219571 | 23.1     | 6658                 | 1.1E+01       |                          |
| HD 221503 | 14.9     | 4241                 | 1.3E-01       | 5.0E+03                  |
| HD 222237 | 11.4     | 4751                 | 2.3E-01       |                          |
| HD 222335 | 18.6     | 5260                 | 4.3E-01       |                          |
| HD 222368 | 13.7     | 6234                 | 3.3E+00       |                          |
| HD 224953 | 15.3     | 4026                 | 7.5E-02       | 6.5E+01                  |
| HD 225213 | 4.3      | 3543                 | 2.2E-02       |                          |
| HD 234078 | 14.2     | 4144                 | 1.1E-01       |                          |
| HD 265866 | 5.6      | 3280                 | 1.6E-02       |                          |
| HIP 171   | 12.1     | 5323                 | 7.1E-01       | 3.7E+00                  |
| HIP 1242  | 6        | 3103                 | 4.3E-03       | 1.8E+00                  |
| HIP 1368  | 15       | 4081                 | 1.1E-01       |                          |
| HIP 2762  | 21.1     | 5983                 | 3.2E+00       | 3.5E-02                  |
| HIP 5496  | 7.8      | 3382                 | 3.8E-02       |                          |
| HIP 13375 | 14.8     | 4057                 | 6.0E-02       |                          |
| HIP 18280 | 15.5     | 4154                 | 1.2E-01       |                          |
| HIP 23452 | 8.6      | 3768                 | 8.0E-02       | 8.6E+00                  |
| HIP 27188 | 13.7     | 4043                 | 9.5E-02       |                          |
| HIP 31634 | 15.3     | 3718                 | 8.0E-02       | 3.3E+01                  |
| HIP 33499 | 8        | 3083                 | 1.5E-02       | 1.0E+01                  |
| HIP 34603 | 6.1      | 3087                 | 1.1E-02       | 5.3E-02                  |
| HIP 37279 | 3.5      | 6600                 | 7.1E+00       | 1.4E+01                  |
| HIP 37288 | 14.5     | 3856                 | 8.0E-02       |                          |
| HIP 37766 | 6        | 3041                 | 9.7E-03       |                          |
| HIP 38382 | 16.5     | 5821                 | 2.0E+00       | 8.7E+00                  |
| HIP 38956 | 8.3      | 3101                 | 8.7E-03       |                          |
| HIP 42220 | 13.9     | 3837                 | 9.3E-02       | 5.7E+00                  |
| HIP 42748 | 15.4     | 3829                 | 8.6E-02       | 1.8E+03                  |

| Name       | $d$ / pc | $T_{\text{eff}}$ / K | $L/L_{\odot}$ | $a_{\text{binary}}$ / au |
|------------|----------|----------------------|---------------|--------------------------|
| HIP 43820  | 11.3     | 3901                 | 1.3E-01       | 7.4E+01                  |
| HIP 44722  | 14.5     | 3850                 | 8.3E-02       |                          |
| HIP 47080  | 11.4     | 5445                 | 7.9E-01       | 4.4E+01                  |
| HIP 49986  | 7.9      | 3488                 | 4.1E-02       |                          |
| HIP 51317  | 7.1      | 3417                 | 2.5E-02       |                          |
| HIP 52600  | 13.9     | 3956                 | 9.0E-02       | 9.3E+00                  |
| HIP 53020  | 6.8      | 3006                 | 8.0E-03       |                          |
| HIP 53767  | 6.7      | 3418                 | 1.9E-02       |                          |
| HIP 54211  | 4.9      | 3638                 | 2.2E-02       | 1.5E+02                  |
| HIP 55203  | 8.4      | 5836                 | 2.3E+00       | 1.6E+00                  |
| HIP 57544  | 5.3      | 3171                 | 7.9E-03       |                          |
| HIP 61094  | 13.7     | 3813                 | 6.3E-02       |                          |
| HIP 61874  | 7.8      | 3144                 | 4.8E-03       |                          |
| HIP 62452  | 8.4      | 3118                 | 1.2E-02       |                          |
| HIP 63366  | 20.9     | 5003                 | 4.1E-01       | 4.3E-01                  |
| HIP 64241  | 17.8     | 6536                 | 5.3E+00       | 1.0E+01                  |
| HIP 65859  | 7.6      | 3566                 | 4.0E-02       |                          |
| HIP 66459  | 10.9     | 3954                 | 6.5E-02       |                          |
| HIP 67090  | 13.2     | 3853                 | 4.6E-02       |                          |
| HIP 70218  | 14.4     | 4255                 | 1.3E-01       |                          |
| HIP 71253  | 6.2      | 3059                 | 9.6E-03       |                          |
| HIP 73470  | 11.9     | 3799                 | 7.3E-02       | 5.0E+00                  |
| HIP 73695  | 12.7     | 5220                 | 1.5E+00       | 3.7E+01                  |
| HIP 76074  | 5.9      | 3365                 | 2.8E-02       |                          |
| HIP 80346  | 8        | 3451                 | 1.9E-02       | 1.7E+00                  |
| HIP 83945  | 7.5      | 3167                 | 8.5E-03       | 5.0E-02                  |
| HIP 86990  | 5.8      | 3184                 | 9.0E-03       |                          |
| HIP 88745  | 15.7     | 5905                 | 2.9E+00       | 1.6E+01                  |
| HIP 93017  | 14.9     | 5891                 | 1.7E+00       | 1.7E+01                  |
| HIP 99461  | 6        | 4871                 | 3.0E-01       | 4.3E+01                  |
| HIP 103039 | 5.7      | 3074                 | 6.5E-03       |                          |
| HIP 105312 | 18       | 5203                 | 8.1E-01       | 1.5E-01                  |
| HIP 106106 | 6.7      | 3346                 | 1.9E-02       | 1.7E-01                  |
| HIP 106255 | 7.8      | 2942                 | 8.7E-03       | 1.1E+00                  |
| HIP 107310 | 22.2     | 6436                 | 6.9E+00       | 4.4E+01                  |
| HIP 110109 | 13.8     | 5685                 | 1.2E+00       | 4.7E+01                  |
| HIP 110778 | 20.2     | 5918                 | 2.0E+00       | 4.5E+01                  |
| HIP 117473 | 6        | 3591                 | 2.6E-02       |                          |
| GJ 55.3    | 21.1     | 6288                 | 4.1E+00       | 1.1E+02                  |
| GJ 83.1    | 4.4      | 2926                 | 2.4E-03       |                          |
| GJ 299     | 6.8      | 2920                 | 2.7E-03       |                          |
| GJ 388     | 4.9      | 3461                 | 2.2E-02       |                          |
| GJ 406     | 2.4      | 2611                 | 6.9E-04       |                          |
| GJ 493.1   | 8.1      | 2943                 | 3.6E-03       |                          |
| GJ 905     | 3.2      | 2950                 | 2.4E-03       |                          |
| GJ 1002    | 4.7      | 2787                 | 1.4E-03       |                          |
| GJ 1057    | 8.5      | 2864                 | 2.9E-03       |                          |
| GJ 1093    | 7.8      | 2742                 | 1.6E-03       |                          |
| GJ 1111    | 3.6      | 2604                 | 7.7E-04       |                          |
| GJ 1151    | 8.2      | 2992                 | 3.4E-03       |                          |
| GJ 1156    | 6.5      | 2817                 | 2.1E-03       |                          |
| GJ 1227    | 8.2      | 2943                 | 3.2E-03       |                          |
| GJ 1286    | 7.2      | 2756                 | 1.4E-03       |                          |
| GJ 1289    | 8.1      | 2998                 | 5.5E-03       |                          |
| GJ 2005    | 7.7      | 2557                 | 1.6E-03       | 8.6E+00                  |
| GJ 3146    | 8.5      | 2688                 | 1.1E-03       |                          |
| GJ 3207    | 7.7      | 3206                 | 8.7E-03       |                          |

| Name     | $d$ / pc | $T_{\text{eff}}$ / K | $L/L_{\odot}$ | $a_{\text{binary}}$ / au |
|----------|----------|----------------------|---------------|--------------------------|
| GJ 3378  | 7.6      | 3101                 | 8.3E-03       |                          |
| GJ 3454  | 8.6      | 2950                 | 5.1E-03       | 7.7E+00                  |
| GJ 3522  | 6.8      | 3159                 | 1.5E-02       | 4.7E-02                  |
| GJ 3622  | 4.5      | 2602                 | 6.8E-04       |                          |
| GJ 3737  | 6.4      | 3012                 | 3.2E-03       |                          |
| GJ 3877  | 6.6      | 2482                 | 7.2E-04       |                          |
| GJ 3959  | 6.4      | 2959                 | 2.8E-03       |                          |
| GJ 4053  | 7.3      | 2951                 | 2.4E-03       |                          |
| GJ 4063  | 7.2      | 3206                 | 2.2E-02       |                          |
| GJ 4248  | 7.4      | 3197                 | 7.4E-03       |                          |
| GJ 4274  | 7.4      | 2911                 | 3.6E-03       |                          |
| LHS 22   | 7        | 2858                 | 2.0E-03       |                          |
| LHS 60   | 5.9      | 3020                 | 3.5E-03       |                          |
| LHS 1565 | 3.7      | 2781                 | 1.6E-03       |                          |
| LHS 1989 | 8        | 3052                 | 8.2E-03       |                          |
| LHS 2090 | 6.4      | 2681                 | 8.4E-04       |                          |
| PLX 2890 | 4.4      | 2806                 | 3.8E-03       | 4.0E+00                  |
| PLX 4459 | 8.2      | 3420                 | 1.4E-02       | 2.4E+00                  |
