# Supplementary material for: No significant correlation between radial velocity planet presence and debris disc properties
Source: arXiv:2005.03573 ancillary file (2020-05-07)
Supplement: Supplementary file 3 [file table3.pdf]

Full version of Table 3

| Name     | Sample | MIPS 70 $\mu\text{m}$          |                                |                                 |        | PACS 70 $\mu\text{m}$          |                                |                                 |        | PACS 100 $\mu\text{m}$         |                                |                                 |        |
|----------|--------|--------------------------------|--------------------------------|---------------------------------|--------|--------------------------------|--------------------------------|---------------------------------|--------|--------------------------------|--------------------------------|---------------------------------|--------|
|          |        | $F_{\nu, \text{obs}}$<br>/ mJy | $\sigma_{\text{obs}}$<br>/ mJy | $F_{\nu, \text{pred}}$<br>/ mJy | $\chi$ | $F_{\nu, \text{obs}}$<br>/ mJy | $\sigma_{\text{obs}}$<br>/ mJy | $F_{\nu, \text{pred}}$<br>/ mJy | $\chi$ | $F_{\nu, \text{obs}}$<br>/ mJy | $\sigma_{\text{obs}}$<br>/ mJy | $F_{\nu, \text{pred}}$<br>/ mJy | $\chi$ |
| HD 142   | P      |                                |                                | 12.96                           |        | 16.05                          | 0.85                           | 13.68                           | 2.78   |                                |                                | 6.75                            |        |
| HD 166   | C      | 105.80                         | 6.32                           | 14.34                           | 14.47  | 96.83                          | 7.71                           | 15.14                           | 10.60  | 65.00                          | 4.21                           | 7.47                            | 13.67  |
| HD 693   | C      | 37.36                          | 4.11                           | 27.95                           | 2.28   |                                |                                | 29.50                           |        | 18.87                          | 1.84                           | 14.46                           | 2.39   |
| HD 739   | C      | 20.11                          | 2.78                           | 17.30                           | 1.01   |                                |                                | 18.26                           |        | 8.63                           | 1.72                           | 8.95                            | -0.19  |
| HD 1237  | P      | 11.81                          | 2.08                           | 9.32                            | 1.19   |                                |                                | 9.84                            |        | 4.10                           | 1.54                           | 4.86                            | -0.49  |
| HD 1326  | P      | 30.50                          | 2.64                           | 30.78                           | -0.10  |                                |                                | 32.52                           |        | 14.74                          | 2.19                           | 16.14                           | -0.64  |
| HD 1461  | P      | 60.39                          | 6.79                           | 8.63                            | 7.63   |                                |                                | 9.11                            |        | 61.13                          | 2.42                           | 4.49                            | 23.42  |
| HD 1581  | C      | 69.96                          | 6.72                           | 59.15                           | 1.60   |                                |                                | 62.45                           |        | 36.13                          | 2.33                           | 30.82                           | 2.25   |
| HD 1835  | C      | 20.46                          | 5.33                           | 8.81                            | 2.18   |                                |                                | 9.31                            |        | 8.40                           | 1.72                           | 4.59                            | 2.22   |
| HD 3443  | C      | 19.23                          | 5.12                           | 22.44                           | -0.62  |                                |                                | 23.69                           |        | 9.38                           | 1.32                           | 11.68                           | -1.73  |
| HD 3651  | P      | 11.78                          | 4.65                           | 21.41                           | -2.07  | 22.14                          | 2.23                           | 22.60                           | -0.20  | 6.28                           | 1.35                           | 11.15                           | -3.59  |
| HD 4203  | P      | -0.62                          | 2.63                           | 1.23                            | -0.70  |                                |                                | 1.30                            |        |                                |                                | 0.64                            |        |
| HD 4208  | P      | 2.71                           | 2.65                           | 2.64                            | 0.03   |                                |                                | 2.79                            |        |                                |                                | 1.38                            |        |
| HD 4308  | P      | 6.69                           | 4.68                           | 8.35                            | -0.36  | 9.87                           | 1.35                           | 8.82                            | 0.78   | 8.29                           | 1.03                           | 4.35                            | 3.83   |
| HD 4391  | C      | 22.41                          | 2.61                           | 15.58                           | 2.62   |                                |                                | 16.44                           |        | 10.61                          | 1.68                           | 8.11                            | 1.49   |
| HD 4628  | C      | 29.58                          | 9.53                           | 31.03                           | -0.15  |                                |                                | 32.76                           |        | 15.34                          | 1.91                           | 16.16                           | -0.43  |
| HD 4676  | C      | 29.80                          | 6.07                           | 23.23                           | 1.08   |                                |                                | 24.52                           |        | 16.65                          | 1.70                           | 12.07                           | 2.69   |
| HD 4747  | C      | 2.08                           | 3.41                           | 6.02                            | -1.15  |                                |                                | 6.36                            |        | 8.76                           | 1.65                           | 3.13                            | 3.42   |
| HD 4813  | C      | 25.54                          | 3.06                           | 21.29                           | 1.39   |                                |                                | 22.47                           |        | 14.05                          | 1.37                           | 11.07                           | 2.16   |
| HD 4967  | C      | 6.91                           | 4.90                           | 4.41                            | 0.51   |                                |                                | 4.65                            |        | -1.36                          | 1.74                           | 2.30                            | -2.11  |
| HD 5133  | C      |                                |                                | 9.12                            |        | 14.35                          | 1.29                           | 9.63                            | 3.64   | 13.97                          | 0.97                           | 4.75                            | 9.52   |
| HD 6434  | P      | 3.35                           | 4.11                           | 2.64                            | 0.17   |                                |                                | 2.78                            |        |                                |                                | 1.37                            |        |
| HD 7439  | C      | 13.97                          | 7.16                           | 19.42                           | -0.76  |                                |                                | 20.50                           |        | 13.43                          | 2.08                           | 10.04                           | 1.63   |
| HD 7570  | C      | 46.54                          | 4.58                           | 25.52                           | 4.59   |                                |                                | 26.94                           |        | 23.15                          | 1.92                           | 13.28                           | 5.13   |
| HD 7924  | P      |                                |                                | 6.85                            |        |                                |                                | 7.23                            |        | 4.87                           | 1.80                           | 3.57                            | 0.72   |
| HD 8574  | P      | 4.78                           | 2.03                           | 3.91                            | 0.43   |                                |                                | 4.13                            |        | 2.83                           | 1.16                           | 2.04                            | 0.69   |
| HD 8673  | P      |                                |                                | 6.54                            |        |                                |                                | 6.90                            |        | 4.07                           | 1.09                           | 3.40                            | 0.61   |
| HD 9540  | C      | -2.26                          | 4.90                           | 6.77                            | -1.84  |                                |                                | 7.15                            |        | 6.42                           | 1.71                           | 3.53                            | 1.69   |
| HD 9826  | P      | 56.34                          | 5.80                           | 56.21                           | 0.02   |                                |                                | 59.34                           |        | 34.53                          | 2.21                           | 29.26                           | 2.37   |
| HD 10307 | C      | 38.86                          | 5.82                           | 32.08                           | 1.16   |                                |                                | 33.86                           |        | 15.69                          | 1.78                           | 16.69                           | -0.56  |
| HD 10361 | C      |                                |                                | 24.30                           |        |                                |                                | 25.66                           |        | 10.73                          | 1.86                           | 12.61                           | -0.91  |
| HD 10476 | C      | 51.25                          | 7.41                           | 38.76                           | 1.68   |                                |                                | 40.92                           |        | 19.40                          | 1.90                           | 20.19                           | -0.41  |
| HD 10647 | P      | 1035.00                        | 52.07                          | 16.47                           | 19.56  | 960.60                         | 55.16                          | 17.39                           | 17.10  | 924.90                         | 53.25                          | 8.53                            | 17.21  |
| HD 10697 | P      | -1.79                          | 2.84                           | 11.25                           | -4.59  |                                |                                | 11.88                           |        | 9.29                           | 1.60                           | 5.86                            | 2.15   |
| HD 10700 | P      | 286.00                         | 28.60                          | 169.09                          | 4.08   | 314.50                         | 18.13                          | 178.51                          | 7.47   |                                |                                | 88.10                           |        |
| HD 11507 | C      | 14.13                          | 2.86                           | 8.36                            | 2.01   | 4.73                           | 1.82                           | 8.83                            | -2.24  | 3.70                           | 0.81                           | 4.36                            | -0.82  |
| HD 11964 | P      | 4.07                           | 3.73                           | 12.46                           | -2.25  |                                |                                | 13.16                           |        | 7.71                           | 1.06                           | 6.49                            | 1.15   |
| HD 12661 | P      | 3.13                           | 4.04                           | 3.61                            | -0.12  |                                |                                | 3.81                            |        | 3.55                           | 1.16                           | 1.88                            | 1.45   |
| HD 13445 | P      | 3.44                           | 5.62                           | 18.06                           | -2.60  | 14.47                          | 1.89                           | 19.07                           | -2.41  | 8.82                           | 1.14                           | 9.40                            | -0.50  |
| HD 13974 | C      | 42.07                          | 5.09                           | 40.24                           | 0.36   |                                |                                | 42.49                           |        | 22.45                          | 1.98                           | 20.92                           | 0.77   |
| HD 14412 | C      | 10.51                          | 2.38                           | 12.20                           | -0.71  |                                |                                | 12.88                           |        | 6.91                           | 0.81                           | 6.35                            | 0.70   |
| HD 16141 | P      | 12.31                          | 5.37                           | 6.19                            | 1.14   |                                |                                | 6.53                            |        | 3.44                           | 1.06                           | 3.22                            | 0.21   |
| HD 16160 | C      | 32.28                          | 6.49                           | 34.31                           | -0.31  |                                |                                | 36.22                           |        | 13.50                          | 1.63                           | 17.87                           | -2.65  |
| HD 16175 | P      | 7.40                           | 3.87                           | 3.61                            | 0.98   |                                |                                | 3.81                            |        | 5.08                           | 1.17                           | 1.88                            | 2.74   |
| HD 16417 | P      |                                |                                | 15.52                           |        |                                |                                | 16.39                           |        | 9.61                           | 1.04                           | 8.08                            | 1.47   |
| HD 16673 | C      | 16.07                          | 5.83                           | 12.09                           | 0.68   |                                |                                | 12.76                           |        | 14.51                          | 1.56                           | 6.29                            | 5.25   |
| HD 16765 | C      | 9.78                           | 6.67                           | 12.75                           | -0.44  |                                |                                | 13.46                           |        | 6.90                           | 2.02                           | 6.60                            | 0.15   |
| HD 17051 | P      | 21.94                          | 3.24                           | 17.25                           | 1.45   |                                |                                | 18.21                           |        | 5.84                           | 1.74                           | 8.98                            | -1.80  |
| HD 17206 | C      | 43.00                          | 16.09                          | 36.48                           | 0.41   |                                |                                | 38.51                           |        | 20.22                          | 1.84                           | 18.95                           | 0.69   |
| HD 17925 | C      | 63.59                          | 6.94                           | 19.83                           | 6.30   | 71.09                          | 3.73                           | 20.93                           | 13.44  | 56.86                          | 3.68                           | 10.33                           | 12.63  |
| HD 19305 | C      | -16.16                         | 5.67                           | 5.16                            | -3.76  |                                |                                | 5.45                            |        | 4.10                           | 1.63                           | 2.69                            | 0.86   |
| HD 20010 | C      | 100.20                         | 7.23                           | 71.65                           | 3.90   |                                |                                | 75.63                           |        | 38.26                          | 2.73                           | 37.08                           | 0.42   |
| HD 20630 | C      | 35.64                          | 7.14                           | 39.11                           | -0.49  |                                |                                | 41.29                           |        | 24.09                          | 2.06                           | 20.35                           | 1.81   |
| HD 20782 | P      | 3.33                           | 2.54                           | 3.66                            | -0.13  |                                |                                | 3.87                            |        | 3.37                           | 1.22                           | 1.91                            | 1.20   |
| HD 20794 | P      | 107.00                         | 6.59                           | 82.17                           | 3.71   | 100.00                         | 5.09                           | 86.75                           | 2.53   | 54.74                          | 2.79                           | 42.82                           | 4.18   |
| HD 20807 | C      |                                |                                | 24.54                           |        | 32.74                          | 2.13                           | 25.91                           | 3.18   | 14.89                          | 1.28                           | 12.77                           | 1.64   |
| HD 21197 | C      | 20.37                          | 5.06                           | 7.23                            | 2.60   |                                |                                | 7.63                            |        | 3.51                           | 1.99                           | 3.77                            | -0.13  |
| HD 21411 | P      | 0.32                           | 4.06                           | 2.78                            | -0.61  |                                |                                | 2.93                            |        |                                |                                | 1.45                            |        |

| Name     | Sample | MIPS 70 $\mu$ m                |                                |                                 |        | PACS 70 $\mu$ m                |                                |                                 |        | PACS 100 $\mu$ m               |                                |                                 |        |
|----------|--------|--------------------------------|--------------------------------|---------------------------------|--------|--------------------------------|--------------------------------|---------------------------------|--------|--------------------------------|--------------------------------|---------------------------------|--------|
|          |        | $F_{\nu, \text{obs}}$<br>/ mJy | $\sigma_{\text{obs}}$<br>/ mJy | $F_{\nu, \text{pred}}$<br>/ mJy | $\chi$ | $F_{\nu, \text{obs}}$<br>/ mJy | $\sigma_{\text{obs}}$<br>/ mJy | $F_{\nu, \text{pred}}$<br>/ mJy | $\chi$ | $F_{\nu, \text{obs}}$<br>/ mJy | $\sigma_{\text{obs}}$<br>/ mJy | $F_{\nu, \text{pred}}$<br>/ mJy | $\chi$ |
| HD 21531 | C      | 8.32                           | 4.94                           | 9.10                            | -0.16  |                                |                                | 9.61                            |        | 3.81                           | 0.83                           | 4.76                            | -1.14  |
| HD 22049 | P      | 1688.00                        | 68.26                          | 180.18                          | 22.09  | 1489.00                        | 84.41                          | 190.22                          | 15.38  |                                |                                | 93.80                           |        |
| HD 22484 | C      | 108.10                         | 7.49                           | 54.45                           | 7.14   | 122.60                         | 8.22                           | 57.48                           | 7.91   | 76.79                          | 6.19                           | 28.34                           | 7.82   |
| HD 22496 | C      | 6.42                           | 4.85                           | 6.68                            | -0.05  |                                |                                | 7.05                            |        | 6.24                           | 1.75                           | 3.49                            | 1.58   |
| HD 23079 | P      | 5.13                           | 1.69                           | 4.04                            | 0.65   |                                |                                | 4.26                            |        | 3.72                           | 1.17                           | 2.10                            | 1.38   |
| HD 23127 | P      | -4.22                          | 2.71                           | 1.16                            | -1.99  |                                |                                | 1.23                            |        |                                |                                | 0.60                            |        |
| HD 23356 | C      | 24.31                          | 5.53                           | 9.04                            | 2.76   | 19.29                          | 2.25                           | 9.54                            | 4.33   | 20.58                          | 2.34                           | 4.71                            | 6.78   |
| HD 23596 | P      | 5.72                           | 2.68                           | 3.47                            | 0.84   |                                |                                | 3.66                            |        | -1.05                          | 1.39                           | 1.80                            | -2.05  |
| HD 23754 | C      | 48.81                          | 3.85                           | 41.82                           | 1.81   |                                |                                | 44.15                           |        | 28.32                          | 2.06                           | 21.72                           | 3.19   |
| HD 26965 | P      | 86.58                          | 5.02                           | 86.07                           | 0.10   |                                |                                | 90.86                           |        | 42.94                          | 2.47                           | 44.85                           | -0.76  |
| HD 27274 | C      | 12.65                          | 4.51                           | 9.10                            | 0.79   | 6.39                           | 1.84                           | 9.61                            | -1.74  | 3.26                           | 0.79                           | 4.73                            | -1.86  |
| HD 27894 | P      | 1.25                           | 2.56                           | 1.21                            | 0.01   |                                |                                | 1.28                            |        |                                |                                | 0.63                            |        |
| HD 28185 | P      | -1.74                          | 1.90                           | 2.66                            | -2.32  |                                |                                | 2.81                            |        |                                |                                | 1.39                            |        |
| HD 30177 | P      | 1.99                           | 2.82                           | 1.64                            | 0.12   |                                |                                | 1.74                            |        |                                |                                | 0.86                            |        |
| HD 30495 | C      | 120.30                         | 7.07                           | 20.00                           | 14.18  | 123.80                         | 7.51                           | 21.12                           | 13.67  | 84.91                          | 5.16                           | 10.41                           | 14.44  |
| HD 30562 | P      |                                |                                | 14.40                           |        |                                |                                | 15.20                           |        | 7.61                           | 1.13                           | 7.49                            | 0.10   |
| HD 30652 | C      | 129.30                         | 8.51                           | 116.81                          | 1.46   |                                |                                | 123.33                          |        | 62.96                          | 3.65                           | 61.05                           | 0.52   |
| HD 32147 | C      | 25.15                          | 3.02                           | 24.94                           | 0.07   |                                |                                | 26.33                           |        | 10.96                          | 1.59                           | 12.99                           | -1.27  |
| HD 33262 | C      | 65.16                          | 5.85                           | 33.08                           | 5.47   |                                |                                | 34.92                           |        | 33.93                          | 2.37                           | 17.13                           | 7.05   |
| HD 33283 | P      | 8.39                           | 3.09                           | 1.75                            | 2.15   |                                |                                | 1.85                            |        |                                |                                | 0.91                            |        |
| HD 33564 | P      | -5.09                          | 5.14                           | 20.71                           | -5.01  |                                |                                | 21.86                           |        | 9.44                           | 1.77                           | 10.77                           | -0.75  |
| HD 33793 | P      | 4.28                           | 3.88                           | 13.02                           | -2.25  |                                |                                | 13.75                           |        | 4.85                           | 1.76                           | 6.83                            | -1.12  |
| HD 34445 | P      |                                |                                | 3.67                            |        |                                |                                | 3.87                            |        | 4.24                           | 3.25                           | 1.91                            | 0.72   |
| HD 36435 | C      | 8.81                           | 4.42                           | 6.41                            | 0.54   |                                |                                | 6.77                            |        | 3.30                           | 1.74                           | 3.34                            | -0.02  |
| HD 36705 | C      | -3.14                          | 6.08                           | 10.80                           | -2.29  |                                |                                | 11.40                           |        | 5.21                           | 1.68                           | 5.58                            | -0.22  |
| HD 37124 | P      | 5.53                           | 3.65                           | 3.32                            | 0.60   |                                |                                | 3.51                            |        | 1.51                           | 1.58                           | 1.73                            | -0.14  |
| HD 37605 | P      | -4.98                          | 5.47                           | 1.48                            | -1.18  |                                |                                | 1.56                            |        |                                |                                | 0.77                            |        |
| HD 38393 | C      | 87.40                          | 5.26                           | 84.40                           | 0.56   |                                |                                | 89.10                           |        | 43.75                          | 4.48                           | 43.83                           | -0.02  |
| HD 38529 | P      | 58.54                          | 7.43                           | 16.20                           | 5.69   | 87.75                          | 3.35                           | 17.11                           | 21.04  |                                |                                | 8.43                            |        |
| HD 39091 | P      | 23.18                          | 3.19                           | 15.59                           | 2.38   | 21.10                          | 1.37                           | 16.45                           | 3.38   | 15.51                          | 1.82                           | 8.11                            | 4.07   |
| HD 39855 | P      | 12.97                          | 6.17                           | 3.97                            | 1.46   |                                |                                | 4.19                            |        |                                |                                | 2.06                            |        |
| HD 40307 | P      | 14.96                          | 4.76                           | 9.86                            | 1.07   | 14.99                          | 1.90                           | 10.41                           | 2.41   | 8.51                           | 0.89                           | 5.13                            | 3.77   |
| HD 40979 | P      | 3.61                           | 2.33                           | 5.26                            | -0.71  |                                |                                | 5.55                            |        | 9.78                           | 1.41                           | 2.73                            | 5.00   |
| HD 41004 | P      | 4.04                           | 2.77                           | 2.29                            | 0.63   |                                |                                | 2.42                            |        | 2.66                           | 1.18                           | 1.19                            | 1.24   |
| HD 42581 | P      | -1.06                          | 2.90                           | 23.08                           | -8.29  |                                |                                | 24.39                           |        | 12.32                          | 1.72                           | 12.16                           | 0.09   |
| HD 43162 | C      | 14.88                          | 2.55                           | 10.40                           | 1.76   |                                |                                | 10.98                           |        | 6.58                           | 0.86                           | 5.42                            | 1.35   |
| HD 43834 | C      | 39.14                          | 5.75                           | 33.89                           | 0.91   |                                |                                | 35.78                           |        | 16.83                          | 1.72                           | 17.64                           | -0.47  |
| HD 45184 | P      | 113.10                         | 8.16                           | 8.78                            | 12.79  | 128.60                         | 5.48                           | 9.27                            | 21.77  |                                |                                | 4.57                            |        |
| HD 45350 | P      | 0.64                           | 3.37                           | 2.54                            | -0.56  |                                |                                | 2.69                            |        |                                |                                | 1.32                            |        |
| HD 46588 | C      | 20.51                          | 2.45                           | 16.64                           | 1.58   |                                |                                | 17.56                           |        | 9.17                           | 1.10                           | 8.63                            | 0.49   |
| HD 48682 | C      | 178.50                         | 9.52                           | 21.75                           | 16.47  | 307.50                         | 12.36                          | 22.97                           | 23.02  | 289.70                         | 17.55                          | 11.31                           | 15.86  |
| HD 49674 | P      | 4.39                           | 2.87                           | 2.11                            | 0.79   |                                |                                | 2.23                            |        |                                |                                | 1.10                            |        |
| HD 50499 | P      | 6.71                           | 2.99                           | 3.58                            | 1.05   |                                |                                | 3.78                            |        | 12.50                          | 1.35                           | 1.86                            | 7.91   |
| HD 50554 | P      | 43.50                          | 3.02                           | 5.13                            | 12.71  | 41.66                          | 1.63                           | 5.41                            | 22.24  | 35.03                          | 1.75                           | 2.67                            | 18.47  |
| HD 50692 | C      | 8.91                           | 4.07                           | 15.06                           | -1.51  | 20.19                          | 2.30                           | 15.90                           | 1.86   | 6.84                           | 0.98                           | 7.84                            | -1.02  |
| HD 52265 | P      | 40.50                          | 6.01                           | 7.94                            | 5.42   | 40.12                          | 4.26                           | 8.38                            | 7.45   | 27.85                          | 2.62                           | 4.13                            | 9.06   |
| HD 52711 | C      | 12.99                          | 3.72                           | 12.87                           | 0.03   |                                |                                | 13.59                           |        | 7.44                           | 0.93                           | 6.70                            | 0.78   |
| HD 53705 | C      | 23.23                          | 2.78                           | 19.20                           | 1.45   |                                |                                | 20.26                           |        | 8.61                           | 3.42                           | 10.00                           | -0.40  |
| HD 55575 | C      | 27.75                          | 4.20                           | 18.41                           | 2.22   |                                |                                | 19.44                           |        | 11.10                          | 1.19                           | 9.58                            | 1.26   |
| HD 58855 | C      | 17.01                          | 3.62                           | 16.84                           | 0.05   |                                |                                | 17.77                           |        | 9.81                           | 1.02                           | 8.71                            | 1.08   |
| HD 60532 | P      |                                |                                | 43.85                           |        | 117.30                         | 22.63                          | 46.29                           | 3.14   | 27.83                          | 2.31                           | 22.71                           | 2.18   |
| HD 61606 | C      | -0.77                          | 5.65                           | 9.20                            | -1.76  |                                |                                | 9.71                            |        | 4.70                           | 1.81                           | 4.79                            | -0.05  |
| HD 62613 | C      | 10.24                          | 2.04                           | 9.04                            | 0.59   | 8.28                           | 1.80                           | 9.55                            | -0.70  | 3.12                           | 0.76                           | 4.71                            | -2.08  |
| HD 63454 | P      | 0.00                           | 2.53                           | 1.32                            | -0.52  |                                |                                | 1.39                            |        |                                |                                | 0.69                            |        |
| HD 65216 | P      | 4.70                           | 2.56                           | 2.33                            | 0.92   |                                |                                | 2.46                            |        |                                |                                | 1.21                            |        |
| HD 66428 | P      | -1.62                          | 2.89                           | 1.73                            | -1.16  |                                |                                | 1.83                            |        |                                |                                | 0.90                            |        |
| HD 68146 | C      | 16.27                          | 2.24                           | 14.35                           | 0.86   |                                |                                | 15.14                           |        | 7.22                           | 3.62                           | 7.43                            | -0.06  |
| HD 68988 | P      | 1.90                           | 2.39                           | 1.58                            | 0.13   |                                |                                | 1.67                            |        |                                |                                | 0.82                            |        |
| HD 69830 | P      | 15.93                          | 2.27                           | 17.66                           | -0.76  |                                |                                | 18.64                           |        | 11.25                          | 1.03                           | 9.20                            | 1.98   |
| HD 69897 | C      | 33.82                          | 5.63                           | 21.99                           | 2.10   |                                |                                | 23.21                           |        | 12.28                          | 2.49                           | 11.37                           | 0.36   |
| HD 70573 | P      | 12.92                          | 3.68                           | 1.08                            | 3.22   |                                |                                | 1.14                            |        | 8.10                           | 4.17                           | 0.56                            | 1.81   |
| HD 71243 | C      | 58.64                          | 4.54                           | 47.45                           | 2.45   |                                |                                | 50.09                           |        | 28.47                          | 2.52                           | 24.62                           | 1.52   |
| HD 72659 | P      | 7.42                           | 2.61                           | 3.17                            | 1.63   |                                |                                | 3.34                            |        | 10.93                          | 1.08                           | 1.65                            | 8.57   |
| HD 72905 | C      | 34.91                          | 3.49                           | 17.39                           | 5.01   |                                |                                | 18.36                           |        | 20.11                          | 1.28                           | 9.05                            | 8.62   |
| HD 73526 | P      | -0.83                          | 9.80                           | 0.92                            | -0.18  |                                |                                | 0.97                            |        |                                |                                | 0.48                            |        |
| HD 74156 | P      | -1.82                          | 3.20                           | 2.61                            | -1.38  |                                |                                | 2.75                            |        |                                |                                | 1.36                            |        |
| HD 75289 | P      | -38.60                         | 19.24                          | 7.37                            | -2.39  |                                |                                | 7.78                            |        |                                |                                | 3.83                            |        |
| HD 75732 | P      | 19.83                          | 3.34                           | 19.27                           | 0.17   |                                |                                | 20.34                           |        | 7.96                           | 1.62                           | 10.03                           | -1.27  |
| HD 76151 | C      | 32.88                          | 3.58                           | 12.62                           | 5.66   |                                |                                | 13.32                           |        | 15.25                          | 1.02                           | 6.56                            | 8.52   |

| Name      | Sample | MIPS 70 $\mu$ m                |                                |                                 |        | PACS 70 $\mu$ m                |                                |                                 |        | PACS 100 $\mu$ m               |                                |                                 |        |
|-----------|--------|--------------------------------|--------------------------------|---------------------------------|--------|--------------------------------|--------------------------------|---------------------------------|--------|--------------------------------|--------------------------------|---------------------------------|--------|
|           |        | $F_{\nu, \text{obs}}$<br>/ mJy | $\sigma_{\text{obs}}$<br>/ mJy | $F_{\nu, \text{pred}}$<br>/ mJy | $\chi$ | $F_{\nu, \text{obs}}$<br>/ mJy | $\sigma_{\text{obs}}$<br>/ mJy | $F_{\nu, \text{pred}}$<br>/ mJy | $\chi$ | $F_{\nu, \text{obs}}$<br>/ mJy | $\sigma_{\text{obs}}$<br>/ mJy | $F_{\nu, \text{pred}}$<br>/ mJy | $\chi$ |
| HD 76700  | P      | 1.84                           | 2.68                           | 1.97                            | -0.05  |                                |                                | 2.08                            |        |                                |                                | 1.02                            |        |
| HD 76932  | C      | 14.64                          | 2.27                           | 14.21                           | 0.19   |                                |                                | 15.00                           |        | 10.90                          | 1.73                           | 7.36                            | 2.04   |
| HD 76943  | C      | 19.54                          | 26.07                          | 55.39                           | -1.37  |                                |                                | 58.47                           |        | 31.96                          | 2.14                           | 28.78                           | 1.46   |
| HD 78154  | C      | 40.41                          | 5.57                           | 30.64                           | 1.75   |                                |                                | 32.34                           |        | 10.97                          | 2.55                           | 15.97                           | -1.96  |
| HD 78366  | C      | 17.34                          | 3.39                           | 12.05                           | 1.56   | 13.53                          | 2.20                           | 12.72                           | 0.37   | 6.15                           | 0.87                           | 6.27                            | -0.13  |
| HD 79028  | C      | 24.59                          | 5.10                           | 26.27                           | -0.33  |                                |                                | 27.73                           |        | 13.60                          | 1.52                           | 13.67                           | -0.04  |
| HD 79096  | C      | 15.72                          | 11.66                          | 10.96                           | 0.41   |                                |                                | 11.57                           |        | 3.63                           | 2.14                           | 5.70                            | -0.97  |
| HD 79210  | C      | 27.73                          | 2.78                           | 27.63                           | 0.03   |                                |                                | 29.18                           |        | 10.09                          | 2.00                           | 14.44                           | -2.17  |
| HD 80606  | P      | 11.27                          | 3.10                           | 0.96                            | 3.33   |                                |                                | 1.02                            |        |                                |                                | 0.50                            |        |
| HD 81040  | P      | 5.55                           | 2.97                           | 2.73                            | 0.95   |                                |                                | 2.89                            |        |                                |                                | 1.42                            |        |
| HD 81997  | C      | 33.84                          | 3.58                           | 31.04                           | 0.78   |                                |                                | 32.77                           |        | 16.16                          | 2.65                           | 16.10                           | 0.02   |
| HD 82106  | C      | -2.19                          | 6.36                           | 8.06                            | -1.61  | 12.34                          | 2.11                           | 8.51                            | 1.82   | 7.57                           | 0.81                           | 4.20                            | 4.14   |
| HD 82328  | C      | 143.60                         | 10.21                          | 131.05                          | 1.21   |                                |                                | 138.34                          |        | 69.55                          | 4.09                           | 67.95                           | 0.38   |
| HD 82943  | P      | 109.80                         | 5.89                           | 6.64                            | 17.50  | 136.40                         | 4.67                           | 7.01                            | 27.71  |                                |                                | 3.45                            |        |
| HD 83443  | P      | -2.34                          | 3.26                           | 2.12                            | -1.37  |                                |                                | 2.24                            |        |                                |                                | 1.10                            |        |
| HD 84117  | C      | 40.25                          | 7.71                           | 27.23                           | 1.69   | 30.36                          | 2.43                           | 28.74                           | 0.66   | 6.90                           | 1.71                           | 14.13                           | -4.22  |
| HD 84737  | C      | 34.94                          | 4.31                           | 27.17                           | 1.80   |                                |                                | 28.68                           |        | 9.12                           | 1.68                           | 14.14                           | -2.98  |
| HD 85512  | P      | 10.20                          | 1.92                           | 11.66                           | -0.76  | 13.29                          | 1.60                           | 12.31                           | 0.61   | 7.14                           | 0.97                           | 6.09                            | 1.08   |
| HD 86728  | C      | -329.50                        | 60.56                          | 22.86                           | -5.82  |                                |                                | 24.14                           |        | 8.93                           | 1.42                           | 11.90                           | -2.08  |
| HD 87883  | P      | -253.00                        | 53.71                          | 5.95                            | -4.82  |                                |                                | 6.28                            |        | 5.77                           | 1.20                           | 3.10                            | 2.23   |
| HD 88133  | P      | 4.79                           | 3.25                           | 2.69                            | 0.64   |                                |                                | 2.84                            |        |                                |                                | 1.40                            |        |
| HD 88230  | C      | 43.21                          | 4.74                           | 51.54                           | -1.74  |                                |                                | 54.41                           |        | 23.14                          | 1.39                           | 26.91                           | -2.64  |
| HD 89125  | C      | 22.76                          | 12.71                          | 12.78                           | 0.78   |                                |                                | 13.49                           |        | 5.64                           | 2.13                           | 6.62                            | -0.46  |
| HD 89269  | C      | -193.20                        | 43.68                          | 7.74                            | -4.60  |                                |                                | 8.17                            |        | 2.83                           | 1.57                           | 4.03                            | -0.76  |
| HD 89307  | P      | -1.44                          | 4.37                           | 4.61                            | -1.38  |                                |                                | 4.86                            |        | 3.74                           | 0.97                           | 2.40                            | 1.39   |
| HD 89449  | C      | 29.10                          | 3.66                           | 25.79                           | 0.90   |                                |                                | 27.23                           |        | 10.79                          | 1.88                           | 13.41                           | -1.39  |
| HD 89744  | P      | 11.74                          | 4.22                           | 12.91                           | -0.28  |                                |                                | 13.63                           |        | 3.90                           | 1.05                           | 6.71                            | -2.67  |
| HD 90089  | C      | 40.94                          | 2.98                           | 15.51                           | 8.51   |                                |                                | 16.37                           |        | 53.36                          | 5.07                           | 8.02                            | 8.94   |
| HD 90156  | P      | 6.79                           | 5.36                           | 6.21                            | 0.11   |                                |                                | 6.56                            |        |                                |                                | 3.23                            |        |
| HD 90839  | C      | 34.01                          | 4.20                           | 29.86                           | 0.98   |                                |                                | 31.53                           |        | 19.39                          | 1.93                           | 15.55                           | 1.98   |
| HD 92788  | P      | 3.57                           | 5.21                           | 3.77                            | -0.04  |                                |                                | 3.98                            |        | 5.17                           | 1.35                           | 1.96                            | 2.39   |
| HD 93083  | P      | 9.46                           | 2.95                           | 2.82                            | 2.25   |                                |                                | 2.98                            |        |                                |                                | 1.47                            |        |
| HD 95128  | P      | 33.02                          | 4.55                           | 27.47                           | 1.22   |                                |                                | 29.00                           |        | 12.39                          | 1.59                           | 14.29                           | -1.19  |
| HD 95735  | P      | 48.23                          | 4.84                           | 56.93                           | -1.78  |                                |                                | 60.14                           |        | 29.25                          | 1.98                           | 29.85                           | -0.30  |
| HD 97101  | C      | 12.23                          | 4.91                           | 9.77                            | 0.50   | 7.85                           | 2.41                           | 10.31                           | -1.02  | 5.62                           | 0.91                           | 5.10                            | 0.57   |
| HD 97584  | C      | 7.12                           | 4.44                           | 7.24                            | -0.03  |                                |                                | 7.64                            |        | 2.99                           | 1.73                           | 3.77                            | -0.45  |
| HD 97658  | P      | 4.99                           | 4.44                           | 4.05                            | 0.21   |                                |                                | 4.28                            |        |                                |                                | 2.11                            |        |
| HD 98712  | C      | 5.49                           | 3.28                           | 8.31                            | -0.86  |                                |                                | 8.77                            |        | 4.60                           | 2.09                           | 4.34                            | 0.13   |
| HD 99492  | P      | 9.35                           | 7.40                           | 6.37                            | 0.40   |                                |                                | 6.72                            |        | 3.78                           | 1.72                           | 3.32                            | 0.27   |
| HD 100180 | C      | 5.21                           | 6.06                           | 8.63                            | -0.56  |                                |                                | 9.11                            |        | 9.31                           | 1.68                           | 4.49                            | 2.87   |
| HD 100623 | C      | 24.91                          | 2.71                           | 20.52                           | 1.62   |                                |                                | 21.66                           |        | 14.16                          | 1.42                           | 10.66                           | 2.46   |
| HD 101177 | C      | 2.15                           | 5.63                           | 7.90                            | -1.02  |                                |                                | 8.34                            |        | 4.62                           | 1.60                           | 4.12                            | 0.31   |
| HD 101501 | C      | 28.50                          | 4.73                           | 28.47                           | 0.01   |                                |                                | 30.06                           |        | 14.63                          | 1.74                           | 14.83                           | -0.11  |
| HD 101581 | C      | 6.97                           | 5.34                           | 7.93                            | -0.18  |                                |                                | 8.37                            |        | 2.30                           | 1.49                           | 4.11                            | -1.21  |
| HD 101930 | P      | -8.74                          | 6.10                           | 2.79                            | -1.89  |                                |                                | 2.95                            |        |                                |                                | 1.45                            |        |
| HD 102117 | P      | -10.43                         | 10.27                          | 3.67                            | -1.37  |                                |                                | 3.88                            |        | 3.62                           | 2.85                           | 1.91                            | 0.60   |
| HD 102195 | P      | 1.37                           | 3.59                           | 2.75                            | -0.38  |                                |                                | 2.90                            |        |                                |                                | 1.43                            |        |
| HD 102365 | P      | 47.80                          | 4.75                           | 39.06                           | 1.84   |                                |                                | 41.24                           |        | 19.30                          | 2.23                           | 20.33                           | -0.46  |
| HD 102438 | C      | 9.79                           | 2.22                           | 9.42                            | 0.17   | 14.01                          | 2.01                           | 9.94                            | 2.02   | 4.85                           | 0.79                           | 4.90                            | -0.06  |
| HD 102870 | C      | 128.90                         | 10.02                          | 95.46                           | 3.33   |                                |                                | 100.78                          |        | 60.20                          | 3.33                           | 49.63                           | 3.15   |
| HD 103095 | C      | 10.10                          | 1.96                           | 14.11                           | -2.03  |                                |                                | 14.89                           |        | 6.62                           | 0.87                           | 7.29                            | -0.77  |
| HD 103932 | C      | 10.16                          | 4.93                           | 16.97                           | -1.38  |                                |                                | 17.92                           |        | 7.86                           | 0.90                           | 8.82                            | -1.06  |
| HD 104067 | P      | 39.59                          | 5.57                           | 4.50                            | 6.29   |                                |                                | 4.75                            |        |                                |                                | 2.35                            |        |
| HD 106252 | P      | 6.23                           | 4.94                           | 3.33                            | 0.59   |                                |                                | 3.52                            |        | 7.84                           | 1.15                           | 1.73                            | 5.32   |
| HD 106516 | C      | 6.40                           | 6.19                           | 8.84                            | -0.39  |                                |                                | 9.33                            |        | 2.79                           | 1.73                           | 4.58                            | -1.04  |
| HD 107148 | P      | -10.31                         | 3.38                           | 2.03                            | -3.65  |                                |                                | 2.14                            |        |                                |                                | 1.06                            |        |
| HD 108147 | P      | -13.00                         | 21.55                          | 3.86                            | -0.78  |                                |                                | 4.07                            |        |                                |                                | 2.00                            |        |
| HD 108874 | P      | 1.74                           | 2.62                           | 1.20                            | 0.20   |                                |                                | 1.27                            |        |                                |                                | 0.63                            |        |
| HD 108954 | C      | 0.00                           | 4.44                           | 8.95                            | -2.02  |                                |                                | 9.45                            |        | 4.04                           | 1.67                           | 4.65                            | -0.37  |
| HD 109358 | C      | 60.03                          | 6.04                           | 60.41                           | -0.06  |                                |                                | 63.78                           |        | 30.57                          | 2.02                           | 31.45                           | -0.43  |
| HD 109749 | P      | -3.24                          | 2.76                           | 1.71                            | -1.79  |                                |                                | 1.80                            |        |                                |                                | 0.89                            |        |
| HD 110315 | C      | 19.92                          | 6.62                           | 7.51                            | 1.87   |                                |                                | 7.93                            |        | 3.40                           | 1.58                           | 3.91                            | -0.33  |
| HD 110833 | C      | 1.31                           | 4.66                           | 10.19                           | -1.91  | 9.73                           | 1.96                           | 10.75                           | -0.52  | 4.38                           | 0.83                           | 5.30                            | -1.11  |
| HD 110897 | C      | 58.48                          | 3.84                           | 12.75                           | 11.90  | 74.84                          | 6.96                           | 13.46                           | 8.82   | 58.42                          | 4.12                           | 6.64                            | 12.58  |
| HD 111232 | P      | -4.27                          | 4.52                           | 3.57                            | -1.74  |                                |                                | 3.77                            |        | 4.36                           | 1.74                           | 1.86                            | 1.44   |
| HD 111395 | C      | 20.44                          | 2.56                           | 11.00                           | 3.68   |                                |                                | 11.62                           |        | 4.79                           | 0.71                           | 5.73                            | -1.31  |
| HD 111631 | C      | 8.77                           | 6.24                           | 10.59                           | -0.29  |                                |                                | 11.19                           |        | 9.97                           | 1.74                           | 5.53                            | 2.55   |
| HD 113337 | P      | 172.30                         | 9.57                           | 7.62                            | 17.21  | 180.80                         | 6.00                           | 8.04                            | 28.79  |                                |                                | 3.96                            |        |
| HD 113538 | P      |                                |                                | 5.28                            |        |                                |                                | 5.58                            |        | -0.69                          | 2.13                           | 2.76                            | -1.62  |

| Name      | Sample | MIPS 70 $\mu\text{m}$         |                                |                                |        | PACS 70 $\mu\text{m}$         |                                |                                |        | PACS 100 $\mu\text{m}$        |                                |                                |        |
|-----------|--------|-------------------------------|--------------------------------|--------------------------------|--------|-------------------------------|--------------------------------|--------------------------------|--------|-------------------------------|--------------------------------|--------------------------------|--------|
|           |        | $F_{\nu,\text{obs}}$<br>/ mJy | $\sigma_{\text{obs}}$<br>/ mJy | $F_{\nu,\text{pred}}$<br>/ mJy | $\chi$ | $F_{\nu,\text{obs}}$<br>/ mJy | $\sigma_{\text{obs}}$<br>/ mJy | $F_{\nu,\text{pred}}$<br>/ mJy | $\chi$ | $F_{\nu,\text{obs}}$<br>/ mJy | $\sigma_{\text{obs}}$<br>/ mJy | $F_{\nu,\text{pred}}$<br>/ mJy | $\chi$ |
| HD 114386 | P      | 6.64                          | 2.66                           | 2.38                           | 1.60   |                               |                                | 2.51                           |        |                               |                                | 1.24                           |        |
| HD 114613 | P      | 57.11                         | 5.19                           | 40.29                          | 3.23   |                               |                                | 42.54                          |        |                               |                                | 20.97                          |        |
| HD 114710 | C      | 50.47                         | 5.95                           | 54.87                          | -0.73  |                               |                                | 57.92                          |        | 23.06                         | 1.82                           | 28.52                          | -2.96  |
| HD 114729 | P      | 8.65                          | 2.27                           | 6.71                           | 0.86   |                               |                                | 7.08                           |        | 5.67                          | 1.18                           | 3.49                           | 1.85   |
| HD 114762 | P      | 0.00                          | 3.06                           | 3.69                           | -1.21  |                               |                                | 3.89                           |        | 3.86                          | 1.01                           | 1.91                           | 1.91   |
| HD 114783 | P      | 5.55                          | 1.97                           | 5.24                           | 0.15   |                               |                                | 5.53                           |        | 5.32                          | 1.07                           | 2.73                           | 2.42   |
| HD 115404 | C      | 9.61                          | 5.42                           | 16.04                          | -1.19  | 15.66                         | 2.09                           | 16.94                          | -0.61  | 8.08                          | 0.88                           | 8.32                           | -0.27  |
| HD 115617 | P      | 153.30                        | 11.27                          | 48.15                          | 9.32   | 219.10                        | 13.22                          | 50.83                          | 12.71  | 181.10                        | 11.24                          | 25.07                          | 13.87  |
| HD 116442 | C      | 6.49                          | 5.88                           | 7.34                           | -0.14  |                               |                                | 7.75                           |        | 4.12                          | 1.79                           | 3.82                           | 0.16   |
| HD 117043 | C      | 22.97                         | 2.50                           | 9.52                           | 5.37   |                               |                                | 10.05                          |        | 9.84                          | 1.89                           | 4.95                           | 2.59   |
| HD 117176 | P      | 40.46                         | 3.74                           | 41.33                          | -0.23  |                               |                                | 43.63                          |        | 46.64                         | 2.63                           | 21.53                          | 9.52   |
| HD 117207 | P      | 4.44                          | 3.17                           | 4.38                           | 0.02   |                               |                                | 4.62                           |        | 3.67                          | 1.07                           | 2.28                           | 1.31   |
| HD 117618 | P      | -0.95                         | 3.06                           | 3.82                           | -1.56  |                               |                                | 4.03                           |        | 2.85                          | 1.27                           | 1.99                           | 0.68   |
| HD 118203 | P      | 6.72                          | 2.85                           | 2.00                           | 1.65   |                               |                                | 2.11                           |        |                               |                                | 1.04                           |        |
| HD 118926 | C      |                               |                                | 3.97                           |        |                               |                                | 4.19                           |        | 5.78                          | 1.93                           | 2.07                           | 1.92   |
| HD 119850 | C      | 18.42                         | 3.38                           | 18.68                          | -0.08  |                               |                                | 19.73                          |        | 8.56                          | 1.61                           | 9.76                           | -0.75  |
| HD 120036 | C      | 10.27                         | 6.13                           | 5.14                           | 0.84   |                               |                                | 5.43                           |        | 3.72                          | 1.69                           | 2.68                           | 0.61   |
| HD 120136 | P      | 32.72                         | 5.78                           | 31.81                          | 0.16   |                               |                                | 33.56                          |        | 20.86                         | 3.45                           | 16.14                          | 1.36   |
| HD 120467 | C      | -3.69                         | 7.05                           | 7.52                           | -1.59  |                               |                                | 7.94                           |        | 4.25                          | 1.68                           | 3.93                           | 0.19   |
| HD 120476 | C      | 2.32                          | 4.74                           | 15.40                          | -2.75  | 10.02                         | 3.13                           | 16.26                          | -1.99  | 5.33                          | 1.18                           | 8.01                           | -2.26  |
| HD 120690 | C      | 8.97                          | 2.79                           | 10.90                          | -0.69  | 8.14                          | 1.86                           | 11.50                          | -1.80  | 5.75                          | 0.90                           | 5.68                           | 0.08   |
| HD 121504 | P      | 0.60                          | 11.01                          | 2.76                           | -0.20  |                               |                                | 2.92                           |        |                               |                                | 1.44                           |        |
| HD 122064 | C      | 17.65                         | 6.65                           | 18.57                          | -0.14  |                               |                                | 19.61                          |        | 9.05                          | 0.92                           | 9.67                           | -0.67  |
| HD 122742 | C      | 4.62                          | 5.49                           | 13.54                          | -1.62  | 15.01                         | 2.06                           | 14.29                          | 0.35   | 6.91                          | 0.83                           | 7.05                           | -0.18  |
| HD 124580 | C      |                               |                                | 8.77                           |        |                               |                                | 9.26                           |        | 9.02                          | 1.64                           | 4.57                           | 2.72   |
| HD 125276 | C      | 15.93                         | 6.20                           | 12.96                          | 0.48   | 14.22                         | 2.62                           | 13.68                          | 0.21   | 3.96                          | 1.30                           | 6.75                           | -2.13  |
| HD 126053 | C      | 5.21                          | 6.04                           | 10.65                          | -0.90  | 13.71                         | 1.92                           | 11.24                          | 1.28   | 3.44                          | 0.75                           | 5.54                           | -2.79  |
| HD 126660 | C      | 70.77                         | 6.26                           | 58.94                          | 1.88   |                               |                                | 62.22                          |        | 33.81                         | 2.90                           | 30.60                          | 1.10   |
| HD 128165 | C      | 33.79                         | 4.99                           | 10.03                          | 4.76   | 15.29                         | 2.01                           | 10.58                          | 2.34   | 10.65                         | 0.84                           | 5.22                           | 6.45   |
| HD 128311 | P      | 22.55                         | 2.14                           | 6.91                           | 7.30   | 24.80                         | 3.01                           | 7.29                           | 5.82   |                               |                                | 3.60                           |        |
| HD 128642 | C      | 6.87                          | 4.51                           | 8.55                           | -0.37  | 9.53                          | 2.27                           | 9.02                           | 0.22   | 5.95                          | 0.90                           | 4.45                           | 1.68   |
| HD 129502 | C      | 55.87                         | 4.60                           | 55.65                          | 0.05   |                               |                                | 58.75                          |        | 36.77                         | 2.39                           | 28.89                          | 3.26   |
| HD 130322 | P      | 1.99                          | 4.97                           | 2.62                           | -0.13  |                               |                                | 2.76                           |        |                               |                                | 1.36                           |        |
| HD 130948 | C      | 11.14                         | 2.99                           | 12.43                          | -0.43  |                               |                                | 13.12                          |        | 6.87                          | 0.79                           | 6.46                           | 0.52   |
| HD 131156 | C      | 69.49                         | 6.82                           | 76.54                          | -1.01  |                               |                                | 80.81                          |        | 36.06                         | 2.80                           | 39.93                          | -1.32  |
| HD 131511 | C      | 35.16                         | 5.86                           | 22.11                          | 2.23   | 30.87                         | 2.17                           | 23.35                          | 3.45   | 21.57                         | 3.93                           | 11.50                          | 2.56   |
| HD 131977 | C      | 52.69                         | 4.13                           | 47.62                          | 1.22   |                               |                                | 50.28                          |        | 22.46                         | 1.60                           | 24.88                          | -1.49  |
| HD 134083 | C      | 36.05                         | 4.76                           | 21.58                          | 3.04   |                               |                                | 22.78                          |        | 7.16                          | 1.35                           | 11.22                          | -2.99  |
| HD 134987 | P      | 4.85                          | 2.80                           | 8.21                           | -1.20  |                               |                                | 8.67                           |        | 5.16                          | 0.91                           | 4.27                           | 0.98   |
| HD 135204 | C      | 6.09                          | 5.97                           | 9.90                           | -0.64  |                               |                                | 10.45                          |        | 6.94                          | 1.70                           | 5.16                           | 1.05   |
| HD 136352 | P      | 18.35                         | 4.01                           | 18.45                          | -0.02  | 21.37                         | 1.68                           | 19.47                          | 1.12   |                               |                                | 9.61                           |        |
| HD 136923 | C      | 11.70                         | 4.58                           | 6.04                           | 1.24   |                               |                                | 6.37                           |        | 4.63                          | 1.75                           | 3.14                           | 0.85   |
| HD 137763 | C      |                               |                                | 8.93                           |        |                               |                                | 9.43                           |        | 4.09                          | 2.34                           | 4.65                           | -0.24  |
| HD 139763 | C      |                               |                                | 4.52                           |        |                               |                                | 4.77                           |        | 3.79                          | 1.61                           | 2.36                           | 0.89   |
| HD 140538 | C      | 12.05                         | 5.72                           | 16.22                          | -0.73  |                               |                                | 17.12                          |        | 9.24                          | 1.36                           | 8.45                           | 0.58   |
| HD 141004 | C      | 52.38                         | 5.74                           | 49.55                          | 0.49   |                               |                                | 52.30                          |        | 29.21                         | 2.11                           | 25.77                          | 1.63   |
| HD 141272 | C      | -17.41                        | 5.48                           | 5.16                           | -4.12  |                               |                                | 5.44                           |        | 2.11                          | 1.62                           | 2.68                           | -0.35  |
| HD 141937 | P      | -1.85                         | 6.94                           | 3.83                           | -0.82  |                               |                                | 4.05                           |        | 5.24                          | 1.45                           | 2.00                           | 2.23   |
| HD 142022 | P      | 7.05                          | 3.16                           | 3.29                           | 1.19   |                               |                                | 3.47                           |        | 2.70                          | 1.27                           | 1.71                           | 0.78   |
| HD 142267 | C      | 10.78                         | 1.81                           | 11.76                          | -0.54  |                               |                                | 12.41                          |        | 5.07                          | 1.64                           | 6.12                           | -0.64  |
| HD 142373 | C      | 40.25                         | 5.93                           | 44.93                          | -0.79  |                               |                                | 47.43                          |        | 19.93                         | 1.82                           | 23.39                          | -1.89  |
| HD 142415 | P      | -6.20                         | 8.63                           | 3.46                           | -1.12  |                               |                                | 3.66                           |        | 7.97                          | 3.52                           | 1.80                           | 1.75   |
| HD 142860 | C      | 73.56                         | 7.48                           | 68.30                          | 0.70   |                               |                                | 72.11                          |        | 33.73                         | 2.26                           | 35.46                          | -0.75  |
| HD 143105 | P      | 5.55                          | 3.62                           | 4.86                           | 0.19   |                               |                                | 5.13                           |        |                               |                                | 2.53                           |        |
| HD 143761 | P      | 30.74                         | 4.41                           | 21.77                          | 2.03   |                               |                                | 22.98                          |        | 9.07                          | 1.20                           | 11.34                          | -1.88  |
| HD 144579 | C      | 12.95                         | 2.92                           | 10.04                          | 1.00   | 9.84                          | 3.30                           | 10.60                          | -0.23  | 3.35                          | 1.12                           | 5.21                           | -1.66  |
| HD 145675 | P      | 10.34                         | 1.92                           | 10.28                          | 0.03   |                               |                                | 10.86                          |        | 5.91                          | 0.99                           | 5.35                           | 0.56   |
| HD 146361 | C      | 28.28                         | 5.41                           | 22.66                          | 1.04   |                               |                                | 23.92                          |        | 10.47                         | 2.17                           | 11.79                          | -0.60  |
| HD 147379 | P      | 17.10                         | 5.13                           | 9.22                           | 1.54   |                               |                                | 9.74                           |        | 1.61                          | 1.93                           | 4.81                           | -1.66  |
| HD 147513 | P      | 11.86                         | 7.42                           | 21.66                          | -1.32  |                               |                                | 22.86                          |        | 14.66                         | 2.24                           | 11.27                          | 1.51   |
| HD 147584 | C      |                               |                                | 30.15                          |        |                               |                                | 31.83                          |        | 14.16                         | 1.60                           | 15.67                          | -0.94  |
| HD 149026 | P      | 0.85                          | 2.58                           | 1.45                           | -0.23  |                               |                                | 1.53                           |        |                               |                                | 0.75                           |        |
| HD 149143 | P      | 5.89                          | 3.06                           | 2.13                           | 1.23   |                               |                                | 2.25                           |        |                               |                                | 1.11                           |        |
| HD 150706 | P      | 43.69                         | 5.09                           | 4.62                           | 7.68   |                               |                                | 4.88                           |        |                               |                                | 2.40                           |        |
| HD 151288 | C      | 16.16                         | 1.84                           | 12.10                          | 2.21   |                               |                                | 12.77                          |        | 4.08                          | 1.65                           | 6.32                           | -1.35  |
| HD 153597 | C      | 47.22                         | 5.47                           | 28.76                          | 3.37   |                               |                                | 30.36                          |        | 15.90                         | 1.13                           | 14.87                          | 0.91   |
| HD 154345 | P      | 5.33                          | 5.09                           | 7.80                           | -0.49  | 6.97                          | 1.14                           | 8.23                           | -1.10  | 3.31                          | 0.81                           | 4.06                           | -0.93  |
| HD 154577 | C      | 21.00                         | 1.47                           | 7.44                           | 9.21   |                               |                                | 7.86                           |        | 11.45                         | 1.77                           | 3.86                           | 4.28   |
| HD 154857 | P      | -1.78                         | 4.70                           | 5.00                           | -1.44  |                               |                                | 5.28                           |        | 2.80                          | 1.38                           | 2.61                           | 0.14   |

| Name       | Sample | MIPS 70 $\mu$ m                |                                |                                 |        | PACS 70 $\mu$ m                |                                |                                 |        | PACS 100 $\mu$ m               |                                |                                 |        |
|------------|--------|--------------------------------|--------------------------------|---------------------------------|--------|--------------------------------|--------------------------------|---------------------------------|--------|--------------------------------|--------------------------------|---------------------------------|--------|
|            |        | $F_{\nu, \text{obs}}$<br>/ mJy | $\sigma_{\text{obs}}$<br>/ mJy | $F_{\nu, \text{pred}}$<br>/ mJy | $\chi$ | $F_{\nu, \text{obs}}$<br>/ mJy | $\sigma_{\text{obs}}$<br>/ mJy | $F_{\nu, \text{pred}}$<br>/ mJy | $\chi$ | $F_{\nu, \text{obs}}$<br>/ mJy | $\sigma_{\text{obs}}$<br>/ mJy | $F_{\nu, \text{pred}}$<br>/ mJy | $\chi$ |
| HD 155358  | P      |                                |                                | 3.75                            |        |                                |                                | 3.95                            |        | 4.00                           | 1.10                           | 1.94                            | 1.86   |
| HD 155876  | C      | 12.34                          | 2.97                           | 14.58                           | -0.75  |                                |                                | 15.40                           |        | 6.61                           | 0.69                           | 7.61                            | -1.43  |
| HD 156668  | P      | 14.51                          | 5.17                           | 3.17                            | 2.19   |                                |                                | 3.35                            |        |                                |                                | 1.65                            |        |
| HD 156846  | P      |                                |                                | 7.04                            |        |                                |                                | 7.44                            |        | 2.78                           | 1.38                           | 3.67                            | -0.64  |
| HD 157214  | C      | 23.92                          | 4.41                           | 23.38                           | 0.12   |                                |                                | 24.69                           |        | 14.24                          | 1.36                           | 12.17                           | 1.51   |
| HD 157881  | C      | 18.33                          | 3.16                           | 23.58                           | -1.66  |                                |                                | 24.90                           |        | 10.17                          | 1.49                           | 12.32                           | -1.43  |
| HD 158633  | C      | 52.83                          | 3.09                           | 12.47                           | 13.04  |                                |                                | 13.16                           |        | 36.15                          | 2.75                           | 6.49                            | 10.78  |
| HD 159868  | P      | -29.39                         | 10.46                          | 4.96                            | -3.28  |                                |                                | 5.24                            |        | -2.32                          | 2.10                           | 2.59                            | -2.33  |
| HD 160032  | C      | 47.44                          | 4.95                           | 25.22                           | 4.48   |                                |                                | 26.63                           |        | 31.04                          | 2.40                           | 13.04                           | 7.48   |
| HD 160691  | P      | 31.52                          | 7.45                           | 28.23                           | 0.44   |                                |                                | 29.80                           |        | 14.55                          | 1.75                           | 14.68                           | -0.08  |
| HD 160922  | C      | 32.13                          | 5.46                           | 25.90                           | 1.14   |                                |                                | 27.34                           |        | 16.32                          | 1.71                           | 13.44                           | 1.68   |
| HD 162004  | P      | -2.15                          | 4.97                           | 11.88                           | -2.82  |                                |                                | 12.54                           |        | 5.04                           | 1.90                           | 6.17                            | -0.59  |
| HD 162020  | P      | -24.07                         | 8.10                           | 2.12                            | -3.24  |                                |                                | 2.24                            |        |                                |                                | 1.10                            |        |
| HD 164922  | P      | 4.97                           | 4.68                           | 6.97                            | -0.43  |                                |                                | 7.35                            |        | 3.61                           | 1.16                           | 3.63                            | -0.02  |
| HD 165499  | C      | 17.95                          | 2.57                           | 18.08                           | -0.05  |                                |                                | 19.09                           |        | 11.28                          | 1.11                           | 9.41                            | 1.67   |
| HD 166348  | C      | 19.24                          | 4.94                           | 6.85                            | 2.51   |                                |                                | 7.24                            |        | 12.72                          | 1.96                           | 3.58                            | 4.67   |
| HD 166620  | C      | 9.30                           | 4.60                           | 16.29                           | -1.52  | 18.29                          | 2.11                           | 17.20                           | 0.51   | 7.79                           | 1.05                           | 8.49                            | -0.67  |
| HD 167425  | C      | 18.43                          | 5.75                           | 9.55                            | 1.54   |                                |                                | 10.08                           |        | 5.00                           | 1.76                           | 4.97                            | 0.01   |
| HD 168151  | C      | 24.49                          | 3.43                           | 22.28                           | 0.64   |                                |                                | 23.52                           |        | 10.24                          | 1.59                           | 11.51                           | -0.79  |
| HD 168443  | P      | -30.62                         | 26.64                          | 6.41                            | -1.39  |                                |                                | 6.76                            |        |                                |                                | 3.34                            |        |
| HD 168746  | P      | 62.79                          | 156.23                         | 2.46                            | 0.39   |                                |                                | 2.60                            |        |                                |                                | 1.28                            |        |
| HD 169830  | P      | 0.82                           | 5.23                           | 10.44                           | -1.84  |                                |                                | 11.02                           |        | 12.42                          | 1.25                           | 5.42                            | 5.60   |
| HD 170153  | C      | 127.60                         | 8.13                           | 106.91                          | 2.53   |                                |                                | 112.87                          |        | 54.88                          | 3.01                           | 55.45                           | -0.19  |
| HD 173739  | C      | 39.20                          | 4.04                           | 23.26                           | 3.86   |                                |                                | 24.59                           |        | 12.11                          | 1.16                           | 12.40                           | -0.22  |
| HD 177565  | P      | 17.74                          | 3.56                           | 12.28                           | 1.53   |                                |                                | 12.96                           |        |                                |                                | 6.39                            |        |
| HD 178911B | P      | 9.43                           | 3.06                           | 3.43                            | 1.96   |                                |                                | 3.62                            |        |                                |                                | 1.78                            |        |
| HD 179930  | C      | -1.76                          | 5.01                           | 5.72                            | -1.49  |                                |                                | 6.04                            |        | 7.56                           | 1.79                           | 2.98                            | 2.55   |
| HD 179949  | P      | -15.34                         | 6.58                           | 7.98                            | -3.54  |                                |                                | 8.43                            |        | 4.16                           | 0.99                           | 4.15                            | 0.00   |
| HD 180161  | C      | 8.62                           | 4.43                           | 6.57                            | 0.46   |                                |                                | 6.94                            |        | 6.41                           | 1.72                           | 3.42                            | 1.73   |
| HD 180617  | P      | 8.43                           | 6.21                           | 18.35                           | -1.60  |                                |                                | 19.39                           |        |                                |                                | 9.65                            |        |
| HD 181321  | C      | 0.51                           | 2.50                           | 8.33                            | -3.12  |                                |                                | 8.80                            |        | 4.62                           | 1.89                           | 4.34                            | 0.15   |
| HD 183263  | P      | 12.25                          | 5.00                           | 2.10                            | 2.03   |                                |                                | 2.22                            |        |                                |                                | 1.09                            |        |
| HD 185269  | P      | 0.00                           | 5.00                           | 6.50                            | -1.30  |                                |                                | 6.87                            |        | 5.04                           | 1.28                           | 3.38                            | 1.29   |
| HD 185395  | C      | 40.27                          | 3.39                           | 31.00                           | 2.72   |                                |                                | 32.72                           |        | 17.03                          | 2.13                           | 16.09                           | 0.44   |
| HD 186427  | P      | -1.13                          | 2.90                           | 10.67                           | -4.07  |                                |                                | 11.26                           |        | 4.27                           | 2.10                           | 5.55                            | -0.61  |
| HD 187085  | P      | 12.87                          | 3.20                           | 3.45                            | 2.94   |                                |                                | 3.64                            |        | 13.83                          | 1.28                           | 1.80                            | 9.40   |
| HD 187123  | P      | 0.45                           | 4.10                           | 2.36                            | -0.47  |                                |                                | 2.49                            |        |                                |                                | 1.23                            |        |
| HD 188015  | P      | 17.53                          | 10.40                          | 1.71                            | 1.52   |                                |                                | 1.81                            |        |                                |                                | 0.89                            |        |
| HD 189245  | C      | 10.59                          | 2.39                           | 13.02                           | -1.01  |                                |                                | 13.74                           |        | 5.38                           | 1.64                           | 6.75                            | -0.84  |
| HD 189567  | C      | 23.52                          | 2.89                           | 12.39                           | 3.85   | 11.21                          | 2.25                           | 13.08                           | -0.83  | 5.15                           | 0.90                           | 6.45                            | -1.44  |
| HD 189733  | P      | 2.00                           | 4.82                           | 5.05                            | -0.63  |                                |                                | 5.33                            |        | 2.91                           | 1.96                           | 2.63                            | 0.14   |
| HD 190007  | C      | 10.49                          | 3.06                           | 10.58                           | -0.03  |                                |                                | 11.17                           |        | 5.56                           | 1.56                           | 5.50                            | 0.04   |
| HD 190422  | C      | -0.38                          | 6.37                           | 8.28                            | -1.36  |                                |                                | 8.75                            |        | 7.96                           | 1.63                           | 4.31                            | 2.24   |
| HD 191849  | C      | 33.79                          | 2.92                           | 21.33                           | 4.25   |                                |                                | 22.52                           |        | 19.35                          | 1.83                           | 11.13                           | 4.48   |
| HD 192263  | P      | 20.50                          | 3.38                           | 4.79                            | 4.64   | 29.56                          | 2.44                           | 5.06                            | 10.03  |                                |                                | 2.48                            |        |
| HD 192310  | P      | 23.74                          | 3.86                           | 28.90                           | -1.33  |                                |                                | 30.51                           |        | 11.51                          | 1.68                           | 15.06                           | -2.10  |
| HD 194640  | C      | 7.18                           | 6.30                           | 8.40                            | -0.19  |                                |                                | 8.87                            |        | 5.15                           | 1.67                           | 4.37                            | 0.47   |
| HD 195019  | P      | 14.40                          | 3.58                           | 6.43                            | 2.23   |                                |                                | 6.79                            |        | 5.30                           | 1.25                           | 3.35                            | 1.55   |
| HD 196050  | P      | 3.22                           | 1.86                           | 3.12                            | 0.05   |                                |                                | 3.30                            |        |                                |                                | 1.63                            |        |
| HD 196761  | C      | 3.73                           | 2.84                           | 11.39                           | -2.70  | 11.71                          | 1.85                           | 12.02                           | -0.17  | 4.79                           | 0.90                           | 5.93                            | -1.25  |
| HD 196877  | C      | 3.55                           | 1.91                           | 6.27                            | -1.42  |                                |                                | 6.62                            |        | -1.47                          | 1.42                           | 3.27                            | -3.33  |
| HD 196885  | P      | 6.87                           | 3.16                           | 6.99                            | -0.04  |                                |                                | 7.38                            |        | 8.17                           | 1.17                           | 3.64                            | 3.87   |
| HD 197076  | C      | 10.10                          | 5.22                           | 8.39                            | 0.33   |                                |                                | 8.86                            |        | 4.80                           | 2.45                           | 4.37                            | 0.17   |
| HD 197692  | C      | 46.81                          | 7.92                           | 44.54                           | 0.29   |                                |                                | 47.02                           |        | 25.43                          | 2.13                           | 23.13                           | 1.07   |
| HD 199260  | C      | 45.26                          | 3.09                           | 12.70                           | 10.54  | 46.65                          | 2.86                           | 13.41                           | 11.62  | 27.19                          | 1.49                           | 6.61                            | 13.78  |
| HD 200525  | C      | 20.34                          | 5.20                           | 18.09                           | 0.43   |                                |                                | 19.09                           |        | 12.70                          | 1.85                           | 9.42                            | 1.77   |
| HD 200779  | C      | 3.09                           | 5.19                           | 6.71                            | -0.70  |                                |                                | 7.08                            |        | 3.08                           | 1.71                           | 3.50                            | -0.24  |
| HD 200968  | C      | -3.04                          | 5.96                           | 7.33                            | -1.74  |                                |                                | 7.74                            |        | 4.19                           | 2.35                           | 3.82                            | 0.16   |
| HD 202206  | P      | 27.91                          | 3.42                           | 2.00                            | 7.58   | 34.19                          | 2.15                           | 2.11                            | 14.92  | 36.94                          | 1.42                           | 1.04                            | 25.21  |
| HD 202275  | C      | 44.34                          | 5.14                           | 39.31                           | 0.98   |                                |                                | 41.49                           |        | 24.58                          | 2.01                           | 20.40                           | 2.07   |
| HD 202560  | C      | 57.35                          | 5.81                           | 66.74                           | -1.61  |                                |                                | 70.48                           |        | 41.64                          | 2.54                           | 34.87                           | 2.64   |
| HD 203244  | C      | -0.31                          | 4.71                           | 6.62                            | -1.47  |                                |                                | 6.99                            |        | 4.72                           | 1.58                           | 3.45                            | 0.81   |
| HD 203608  | C      | 51.86                          | 6.63                           | 54.25                           | -0.36  |                                |                                | 57.27                           |        | 31.76                          | 2.31                           | 28.04                           | 1.59   |
| HD 204961  | P      | 22.62                          | 5.08                           | 21.17                           | 0.28   |                                |                                | 22.36                           |        | 14.39                          | 1.62                           | 11.10                           | 2.02   |
| HD 205390  | C      | 11.52                          | 5.33                           | 8.32                            | 0.60   | 13.84                          | 1.81                           | 8.79                            | 2.78   | 4.31                           | 0.80                           | 4.32                            | -0.01  |
| HD 207129  | C      | 365.80                         | 19.59                          | 17.25                           | 17.79  | 316.10                         | 27.67                          | 18.21                           | 10.76  | 342.50                         | 19.87                          | 8.97                            | 16.78  |
| HD 208487  | P      | -2.18                          | 2.96                           | 2.58                            | -1.61  |                                |                                | 2.72                            |        |                                |                                | 1.34                            |        |
| HD 209100  | C      | 111.60                         | 8.24                           | 116.37                          | -0.57  |                                |                                | 122.86                          |        | 58.73                          | 2.94                           | 60.61                           | -0.63  |
| HD 209458  | P      | -9.28                          | 3.13                           | 2.34                            | -3.71  |                                |                                | 2.47                            |        |                                |                                | 1.22                            |        |

| Name      | Sample | MIPS 70 $\mu$ m                |                                |                                 |        | PACS 70 $\mu$ m                |                                |                                 |        | PACS 100 $\mu$ m               |                                |                                 |        |
|-----------|--------|--------------------------------|--------------------------------|---------------------------------|--------|--------------------------------|--------------------------------|---------------------------------|--------|--------------------------------|--------------------------------|---------------------------------|--------|
|           |        | $F_{\nu, \text{obs}}$<br>/ mJy | $\sigma_{\text{obs}}$<br>/ mJy | $F_{\nu, \text{pred}}$<br>/ mJy | $\chi$ | $F_{\nu, \text{obs}}$<br>/ mJy | $\sigma_{\text{obs}}$<br>/ mJy | $F_{\nu, \text{pred}}$<br>/ mJy | $\chi$ | $F_{\nu, \text{obs}}$<br>/ mJy | $\sigma_{\text{obs}}$<br>/ mJy | $F_{\nu, \text{pred}}$<br>/ mJy | $\chi$ |
| HD 210027 | C      | 71.16                          | 6.35                           | 68.83                           | 0.36   |                                |                                | 72.66                           |        | 34.11                          | 2.25                           | 35.69                           | -0.69  |
| HD 210277 | P      | 10.25                          | 2.06                           | 8.79                            | 0.71   |                                |                                | 9.27                            |        | 8.18                           | 1.02                           | 4.57                            | 3.52   |
| HD 210302 | C      | 8.61                           | 5.71                           | 23.55                           | -2.62  |                                |                                | 24.86                           |        | 12.02                          | 1.54                           | 12.25                           | -0.15  |
| HD 211970 | P      | 11.30                          | 5.79                           | 5.21                            | 1.05   |                                |                                | 5.50                            |        | 4.47                           | 1.58                           | 2.72                            | 1.11   |
| HD 212301 | P      | 2.86                           | 2.81                           | 2.21                            | 0.23   |                                |                                | 2.33                            |        |                                |                                | 1.15                            |        |
| HD 212330 | C      | 26.00                          | 4.53                           | 26.25                           | -0.05  |                                |                                | 27.71                           |        | 11.50                          | 1.67                           | 13.66                           | -1.29  |
| HD 213240 | P      | 6.28                           | 1.69                           | 5.53                            | 0.44   |                                |                                | 5.84                            |        | 5.28                           | 1.18                           | 2.88                            | 2.04   |
| HD 213845 | C      | 25.22                          | 3.22                           | 16.97                           | 2.56   |                                |                                | 17.91                           |        | 15.82                          | 1.79                           | 8.80                            | 3.91   |
| HD 214749 | C      | 8.22                           | 5.89                           | 7.82                            | 0.07   |                                |                                | 8.26                            |        | 2.50                           | 1.54                           | 4.07                            | -1.02  |
| HD 214953 | C      | 6.82                           | 5.25                           | 11.09                           | -0.81  |                                |                                | 11.71                           |        | 2.77                           | 2.09                           | 5.77                            | -1.43  |
| HD 215152 | P      | 18.80                          | 5.62                           | 4.15                            | 2.61   |                                |                                | 4.38                            |        |                                |                                | 2.16                            |        |
| HD 215648 | C      | 54.65                          | 4.59                           | 53.81                           | 0.18   |                                |                                | 56.80                           |        | 26.02                          | 2.12                           | 27.87                           | -0.86  |
| HD 216133 | C      |                                |                                | 4.05                            |        |                                |                                | 4.27                            |        | 2.55                           | 1.62                           | 2.11                            | 0.27   |
| HD 216435 | P      | 42.93                          | 3.97                           | 10.72                           | 8.11   | 51.11                          | 2.80                           | 11.31                           | 14.19  |                                |                                | 5.58                            |        |
| HD 216437 | P      | 9.28                           | 2.91                           | 11.55                           | -0.78  |                                |                                | 12.20                           |        | 5.94                           | 1.04                           | 6.01                            | -0.06  |
| HD 216770 | P      | 3.67                           | 2.99                           | 2.39                            | 0.43   |                                |                                | 2.52                            |        |                                |                                | 1.24                            |        |
| HD 216899 | C      | 18.27                          | 3.50                           | 16.77                           | 0.43   |                                |                                | 17.71                           |        | 6.56                           | 1.62                           | 8.74                            | -1.34  |
| HD 217014 | P      | 26.79                          | 4.94                           | 19.95                           | 1.39   |                                |                                | 21.06                           |        | 13.11                          | 3.36                           | 10.38                           | 0.81   |
| HD 217107 | P      | 6.32                           | 5.64                           | 11.96                           | -1.00  |                                |                                | 12.62                           |        | 2.65                           | 1.64                           | 6.22                            | -2.18  |
| HD 217357 | C      | 21.74                          | 2.61                           | 15.36                           | 2.44   |                                |                                | 16.22                           |        | 10.16                          | 1.10                           | 8.02                            | 1.94   |
| HD 217987 | C      | 54.30                          | 5.38                           | 52.19                           | 0.39   |                                |                                | 55.12                           |        | 28.80                          | 2.13                           | 27.28                           | 0.70   |
| HD 218511 | C      | 0.30                           | 5.09                           | 6.14                            | -1.15  | 12.26                          | 1.06                           | 6.49                            | 5.43   | 15.73                          | 1.81                           | 3.21                            | 6.92   |
| HD 219134 | P      | 17.59                          | 8.18                           | 42.47                           | -3.03  |                                |                                | 44.84                           |        |                                |                                | 22.12                           |        |
| HD 219482 | C      | 72.65                          | 4.07                           | 13.60                           | 14.50  | 69.76                          | 4.69                           | 14.36                           | 11.80  | 40.06                          | 2.05                           | 7.04                            | 16.09  |
| HD 219571 | C      | 54.46                          | 5.63                           | 49.46                           | 0.86   |                                |                                | 52.21                           |        | 33.57                          | 2.24                           | 25.62                           | 3.41   |
| HD 221420 | P      | 17.44                          | 2.83                           | 14.94                           | 0.88   |                                |                                | 15.77                           |        |                                |                                | 7.77                            |        |
| HD 221503 | C      | 18.40                          | 5.73                           | 5.96                            | 2.17   |                                |                                | 6.29                            |        | 0.21                           | 1.78                           | 3.11                            | -1.62  |
| HD 222237 | C      | 15.92                          | 1.94                           | 11.65                           | 2.19   |                                |                                | 12.30                           |        | 5.13                           | 0.83                           | 6.07                            | -1.13  |
| HD 222335 | C      | 0.86                           | 5.51                           | 6.39                            | -1.00  |                                |                                | 6.74                            |        | 2.69                           | 1.66                           | 3.33                            | -0.38  |
| HD 222368 | C      | 70.05                          | 6.43                           | 55.28                           | 2.29   |                                |                                | 58.35                           |        | 42.62                          | 2.58                           | 28.74                           | 5.34   |
| HD 222582 | P      | -1.25                          | 2.19                           | 2.75                            | -1.82  |                                |                                | 2.90                            |        |                                |                                | 1.43                            |        |
| HD 224693 | P      | 7.15                           | 2.65                           | 1.51                            | 2.13   |                                |                                | 1.59                            |        |                                |                                | 0.78                            |        |
| HD 224953 | C      | -1.39                          | 4.93                           | 3.57                            | -1.00  |                                |                                | 3.76                            |        | 3.26                           | 2.25                           | 1.86                            | 0.62   |
| HD 225213 | C      | 15.52                          | 4.36                           | 20.13                           | -1.05  |                                |                                | 21.26                           |        | 9.58                           | 1.68                           | 10.54                           | -0.57  |
| HD 234078 | C      | 10.88                          | 5.13                           | 5.78                            | 0.99   |                                |                                | 6.10                            |        | 0.84                           | 1.59                           | 3.02                            | -1.36  |
| HD 265866 | C      |                                |                                | 11.63                           |        |                                |                                | 12.29                           |        | 5.29                           | 1.55                           | 6.13                            | -0.54  |
| HD 285968 | P      |                                |                                | 7.39                            |        |                                |                                | 7.80                            |        | 3.66                           | 1.66                           | 3.87                            | -0.13  |
| HD 330075 | P      | 11.81                          | 12.44                          | 1.10                            | 0.86   |                                |                                | 1.16                            |        |                                |                                | 0.57                            |        |
| HIP 171   | C      | 27.45                          | 5.11                           | 23.13                           | 0.84   |                                |                                | 24.42                           |        | 12.73                          | 1.13                           | 11.98                           | 0.65   |
| HIP 1242  | C      |                                |                                | 4.63                            |        |                                |                                | 4.89                            |        | -0.39                          | 1.64                           | 2.48                            | -1.75  |
| HIP 1368  | C      | 20.38                          | 5.15                           | 5.58                            | 2.87   | 17.49                          | 3.39                           | 5.89                            | 3.42   | 40.92                          | 6.01                           | 2.91                            | 6.32   |
| HIP 2762  | C      | 21.17                          | 6.11                           | 23.81                           | -0.43  |                                |                                | 25.13                           |        | 18.25                          | 1.95                           | 12.40                           | 2.98   |
| HIP 5496  | C      | 8.16                           | 3.08                           | 11.60                           | -1.11  |                                |                                | 12.25                           |        | 6.93                           | 1.48                           | 6.08                            | 0.58   |
| HIP 5643  | P      | 5.80                           | 1.63                           | 4.79                            | 0.62   |                                |                                | 5.06                            |        | 6.59                           | 1.71                           | 2.63                            | 2.32   |
| HIP 12961 | P      | 6.46                           | 3.93                           | 1.83                            | 1.18   |                                |                                | 1.94                            |        |                                |                                | 0.96                            |        |
| HIP 13375 | C      |                                |                                | 3.11                            |        |                                |                                | 3.29                            |        | 2.45                           | 1.58                           | 1.62                            | 0.52   |
| HIP 14810 | P      | -5.79                          | 3.16                           | 1.48                            | -2.30  |                                |                                | 1.56                            |        |                                |                                | 0.77                            |        |
| HIP 18280 | C      | 7.18                           | 6.02                           | 4.97                            | 0.37   |                                |                                | 5.25                            |        | 4.43                           | 1.85                           | 2.59                            | 1.00   |
| HIP 19165 | P      | 2.56                           | 3.86                           | 1.80                            | 0.20   |                                |                                | 1.90                            |        |                                |                                | 0.94                            |        |
| HIP 22627 | P      |                                |                                | 2.69                            |        |                                |                                | 2.84                            |        | -1.64                          | 1.22                           | 1.43                            | -2.52  |
| HIP 23452 | C      | 14.06                          | 3.12                           | 15.70                           | -0.52  |                                |                                | 16.58                           |        | 9.65                           | 1.64                           | 8.19                            | 0.89   |
| HIP 27188 | C      | 5.41                           | 5.12                           | 5.91                            | -0.10  |                                |                                | 6.24                            |        | 5.12                           | 1.67                           | 3.08                            | 1.22   |
| HIP 31634 | C      |                                |                                | 5.22                            |        |                                |                                | 5.51                            |        | 2.26                           | 1.80                           | 2.73                            | -0.26  |
| HIP 33499 | C      |                                |                                | 6.43                            |        |                                |                                | 6.79                            |        | 1.48                           | 1.67                           | 3.41                            | -1.16  |
| HIP 34603 | C      |                                |                                | 7.43                            |        |                                |                                | 7.85                            |        | 5.02                           | 1.59                           | 3.93                            | 0.68   |
| HIP 36208 | P      | 12.27                          | 3.55                           | 17.37                           | -1.44  |                                |                                | 18.36                           |        | 7.79                           | 1.73                           | 9.26                            | -0.85  |
| HIP 37279 | C      |                                |                                | 1441.52                         |        |                                |                                | 1521.74                         |        | 834.00                         | 39.96                          | 749.13                          | 2.08   |
| HIP 37288 | C      |                                |                                | 4.70                            |        |                                |                                | 4.96                            |        | 4.56                           | 1.56                           | 2.45                            | 1.36   |
| HIP 37766 | C      | 11.96                          | 3.24                           | 7.54                            | 1.36   |                                |                                | 7.98                            |        | 8.95                           | 1.72                           | 4.08                            | 2.83   |
| HIP 38382 | C      | 17.08                          | 5.57                           | 26.54                           | -1.70  |                                |                                | 28.01                           |        | 14.83                          | 1.57                           | 13.81                           | 0.64   |
| HIP 38956 | C      |                                |                                | 2.99                            |        |                                |                                | 3.16                            |        | -0.95                          | 1.59                           | 1.60                            | -1.60  |
| HIP 42220 | C      |                                |                                | 6.38                            |        |                                |                                | 6.73                            |        | 4.45                           | 1.73                           | 3.33                            | 0.65   |
| HIP 42748 | C      |                                |                                | 4.87                            |        |                                |                                | 5.14                            |        | 5.03                           | 1.79                           | 2.54                            | 1.39   |
| HIP 43790 | P      | -13.24                         | 4.86                           | 2.84                            | -3.31  |                                |                                | 3.00                            |        |                                |                                | 1.48                            |        |
| HIP 43820 | C      |                                |                                | 13.30                           |        |                                |                                | 14.04                           |        | 6.69                           | 1.75                           | 6.94                            | -0.14  |
| HIP 44722 | C      |                                |                                | 5.29                            |        |                                |                                | 5.59                            |        | 3.04                           | 1.47                           | 2.76                            | 0.19   |
| HIP 47080 | C      | -87.13                         | 51.91                          | 28.47                           | -2.23  |                                |                                | 30.05                           |        | 12.53                          | 1.79                           | 14.82                           | -1.28  |
| HIP 49986 | C      | 2.45                           | 3.23                           | 12.79                           | -3.20  |                                |                                | 13.51                           |        | 6.91                           | 1.62                           | 6.71                            | 0.12   |
| HIP 51317 | C      | 6.62                           | 4.26                           | 10.11                           | -0.82  |                                |                                | 10.68                           |        | 4.91                           | 1.69                           | 5.32                            | -0.24  |

| Name       | Sample | MIPS 70 $\mu$ m                |                                |                                 |        | PACS 70 $\mu$ m                |                                |                                 |        | PACS 100 $\mu$ m               |                                |                                 |        |
|------------|--------|--------------------------------|--------------------------------|---------------------------------|--------|--------------------------------|--------------------------------|---------------------------------|--------|--------------------------------|--------------------------------|---------------------------------|--------|
|            |        | $F_{\nu, \text{obs}}$<br>/ mJy | $\sigma_{\text{obs}}$<br>/ mJy | $F_{\nu, \text{pred}}$<br>/ mJy | $\chi$ | $F_{\nu, \text{obs}}$<br>/ mJy | $\sigma_{\text{obs}}$<br>/ mJy | $F_{\nu, \text{pred}}$<br>/ mJy | $\chi$ | $F_{\nu, \text{obs}}$<br>/ mJy | $\sigma_{\text{obs}}$<br>/ mJy | $F_{\nu, \text{pred}}$<br>/ mJy | $\chi$ |
| HIP 52600  | C      | -2.45                          | 5.85                           | 5.85                            | -1.42  |                                |                                | 6.18                            |        | 2.08                           | 1.58                           | 3.06                            | -0.61  |
| HIP 53020  | C      |                                |                                | 4.84                            |        |                                |                                | 5.12                            |        | 0.68                           | 1.44                           | 2.61                            | -1.33  |
| HIP 53767  | C      | 14.96                          | 3.87                           | 8.44                            | 1.68   |                                |                                | 8.92                            |        | 4.90                           | 1.42                           | 4.42                            | 0.34   |
| HIP 54211  | C      | 20.27                          | 4.41                           | 15.05                           | 1.18   |                                |                                | 15.90                           |        | 6.64                           | 2.14                           | 7.86                            | -0.57  |
| HIP 55203  | C      |                                |                                | 106.83                          |        |                                |                                | 112.80                          |        | 57.12                          | 3.18                           | 55.93                           | 0.33   |
| HIP 56528  | P      |                                |                                | 7.57                            |        |                                |                                | 8.00                            |        | 11.87                          | 1.29                           | 3.97                            | 6.11   |
| HIP 57050  | P      |                                |                                | 3.17                            |        |                                |                                | 3.35                            |        | 1.47                           | 1.00                           | 1.68                            | -0.21  |
| HIP 57087  | P      | 3.93                           | 1.72                           | 4.95                            | -0.59  |                                |                                | 5.23                            |        | 3.52                           | 1.11                           | 2.59                            | 0.84   |
| HIP 57544  | C      |                                |                                | 7.14                            |        |                                |                                | 7.54                            |        | 2.67                           | 1.96                           | 3.80                            | -0.58  |
| HIP 57548  | P      | 7.50                           | 5.01                           | 9.35                            | -0.37  |                                |                                | 9.89                            |        | 2.45                           | 1.95                           | 5.09                            | -1.36  |
| HIP 61094  | C      |                                |                                | 4.77                            |        |                                |                                | 5.03                            |        | 2.72                           | 1.48                           | 2.49                            | 0.16   |
| HIP 61874  | C      |                                |                                | 1.87                            |        |                                |                                | 1.98                            |        | 5.36                           | 1.85                           | 1.00                            | 2.35   |
| HIP 62452  | C      |                                |                                | 4.89                            |        |                                |                                | 5.16                            |        | 5.51                           | 1.74                           | 2.60                            | 1.67   |
| HIP 63366  | C      | -5.42                          | 5.19                           | 5.06                            | -2.02  |                                |                                | 5.34                            |        | -0.43                          | 1.71                           | 2.62                            | -1.78  |
| HIP 64241  | C      | 51.60                          | 5.72                           | 43.02                           | 1.48   |                                |                                | 45.43                           |        | 24.97                          | 1.96                           | 22.58                           | 1.17   |
| HIP 65859  | C      | 14.54                          | 3.97                           | 11.94                           | 0.65   |                                |                                | 12.62                           |        | 7.17                           | 1.73                           | 6.26                            | 0.52   |
| HIP 66459  | C      |                                |                                | 6.63                            |        |                                |                                | 7.00                            |        | 2.20                           | 1.40                           | 3.46                            | -0.90  |
| HIP 67090  | C      |                                |                                | 3.71                            |        |                                |                                | 3.92                            |        | 1.70                           | 1.53                           | 1.94                            | -0.16  |
| HIP 70218  | C      | 9.73                           | 4.88                           | 6.09                            | 0.75   |                                |                                | 6.43                            |        | 3.01                           | 1.63                           | 3.18                            | -0.11  |
| HIP 70849  | P      |                                |                                | 1.88                            |        |                                |                                | 1.98                            |        | 1.69                           | 1.43                           | 0.98                            | 0.50   |
| HIP 70890  | P      | -37.06                         | 23.19                          | 31.32                           | -2.95  |                                |                                | 33.12                           |        |                                |                                | 17.36                           |        |
| HIP 71253  | C      |                                |                                | 6.94                            |        |                                |                                | 7.34                            |        | 4.87                           | 1.46                           | 3.71                            | 0.80   |
| HIP 73470  | C      |                                |                                | 7.44                            |        |                                |                                | 7.86                            |        | 4.81                           | 1.59                           | 3.88                            | 0.58   |
| HIP 73695  | C      | 72.62                          | 6.03                           | 49.71                           | 3.78   |                                |                                | 52.48                           |        | 30.70                          | 2.15                           | 26.13                           | 2.10   |
| HIP 74995  | P      | 17.57                          | 3.12                           | 7.18                            | 3.33   | 15.26                          | 1.02                           | 7.59                            | 7.52   | 11.83                          | 1.85                           | 3.82                            | 4.34   |
| HIP 76074  | C      | 18.92                          | 4.26                           | 16.80                           | 0.50   |                                |                                | 17.75                           |        | 5.50                           | 1.75                           | 8.83                            | -1.90  |
| HIP 80346  | C      |                                |                                | 5.97                            |        |                                |                                | 6.31                            |        | 3.27                           | 1.55                           | 3.13                            | 0.09   |
| HIP 80459  | P      |                                |                                | 6.66                            |        |                                |                                | 7.03                            |        | 4.97                           | 1.71                           | 3.50                            | 0.86   |
| HIP 80824  | P      | 20.27                          | 3.93                           | 14.85                           | 1.38   |                                |                                | 15.70                           |        |                                |                                | 7.93                            |        |
| HIP 83043  | P      |                                |                                | 7.06                            |        |                                |                                | 7.45                            |        | 22.34                          | 2.46                           | 3.69                            | 7.57   |
| HIP 83945  | C      |                                |                                | 3.96                            |        |                                |                                | 4.18                            |        | -2.34                          | 1.79                           | 2.09                            | -2.48  |
| HIP 85523  | P      | 31.08                          | 9.57                           | 15.51                           | 1.63   | 16.02                          | 1.71                           | 16.39                           | -0.22  |                                |                                | 8.14                            |        |
| HIP 85647  | P      |                                |                                | 4.81                            |        |                                |                                | 5.08                            |        | 0.97                           | 1.09                           | 2.51                            | -1.40  |
| HIP 86162  | P      | 26.09                          | 4.44                           | 19.72                           | 1.43   |                                |                                | 20.83                           |        | 5.90                           | 1.63                           | 10.29                           | -2.68  |
| HIP 86214  | P      | -6.93                          | 9.74                           | 8.87                            | -1.62  |                                |                                | 9.38                            |        |                                |                                | 4.78                            |        |
| HIP 86287  | P      |                                |                                | 7.91                            |        |                                |                                | 8.36                            |        | 2.39                           | 1.68                           | 4.15                            | -1.05  |
| HIP 86990  | C      |                                |                                | 6.38                            |        |                                |                                | 6.74                            |        | 3.01                           | 1.59                           | 3.41                            | -0.25  |
| HIP 88745  | C      | 96.93                          | 7.09                           | 29.32                           | 9.52   | 108.20                         | 7.40                           | 30.95                           | 10.42  | 105.80                         | 7.30                           | 15.20                           | 12.41  |
| HIP 93017  | C      | 26.65                          | 5.26                           | 27.50                           | -0.16  |                                |                                | 29.04                           |        | 17.48                          | 1.87                           | 14.42                           | 1.61   |
| HIP 99461  | C      | 50.65                          | 8.89                           | 51.25                           | -0.07  |                                |                                | 54.11                           |        | 24.83                          | 1.93                           | 26.58                           | -0.88  |
| HIP 103039 | C      |                                |                                | 5.72                            |        |                                |                                | 6.05                            |        | 3.48                           | 1.60                           | 3.05                            | 0.27   |
| HIP 105312 | C      | 10.99                          | 6.74                           | 12.50                           | -0.22  | 11.80                          | 2.09                           | 13.19                           | -0.66  | 9.74                           | 1.04                           | 6.51                            | 3.03   |
| HIP 106106 | C      | 9.42                           | 3.33                           | 9.06                            | 0.11   |                                |                                | 9.57                            |        | 4.37                           | 1.54                           | 4.75                            | -0.25  |
| HIP 106255 | C      |                                |                                | 4.86                            |        |                                |                                | 5.14                            |        | 3.25                           | 1.60                           | 2.64                            | 0.38   |
| HIP 107310 | C      | 39.36                          | 5.18                           | 37.72                           | 0.31   |                                |                                | 39.83                           |        | 22.27                          | 2.12                           | 19.69                           | 1.17   |
| HIP 109388 | P      | 1.54                           | 2.84                           | 7.87                            | -2.23  |                                |                                | 8.32                            |        | 4.34                           | 1.19                           | 4.13                            | 0.17   |
| HIP 110109 | C      | 25.50                          | 5.73                           | 24.44                           | 0.19   |                                |                                | 25.80                           |        | 9.13                           | 1.41                           | 12.72                           | -2.52  |
| HIP 110778 | C      |                                |                                | 18.60                           |        |                                |                                | 19.64                           |        | 6.24                           | 1.77                           | 9.68                            | -1.89  |
| HIP 113020 | P      | 7.95                           | 2.61                           | 15.07                           | -2.72  |                                |                                | 15.93                           |        | 6.54                           | 1.62                           | 8.02                            | -0.92  |
| HIP 117473 | C      | 12.18                          | 1.94                           | 12.47                           | -0.15  |                                |                                | 13.17                           |        | 4.22                           | 1.69                           | 6.52                            | -1.36  |
| GJ 55.3    | C      |                                |                                | 26.68                           |        |                                |                                | 28.16                           |        | 9.44                           | 2.20                           | 13.85                           | -1.96  |
| GJ 83.1    | C      | 1.07                           | 3.27                           | 3.69                            | -0.80  |                                |                                | 3.90                            |        | -2.93                          | 1.57                           | 2.03                            | -3.16  |
| GJ 299     | C      |                                |                                | 1.69                            |        |                                |                                | 1.79                            |        | 5.26                           | 1.63                           | 0.93                            | 2.65   |
| GJ 317     | P      |                                |                                | 2.34                            |        |                                |                                | 2.48                            |        | 3.29                           | 1.12                           | 1.24                            | 1.83   |
| GJ 388     | C      | 11.15                          | 2.97                           | 17.12                           | -2.00  |                                |                                | 18.08                           |        | 5.05                           | 1.75                           | 8.94                            | -2.23  |
| GJ 406     | C      |                                |                                | 4.97                            |        |                                |                                | 5.25                            |        | 4.99                           | 1.62                           | 2.78                            | 1.37   |
| GJ 493.1   | C      |                                |                                | 1.54                            |        |                                |                                | 1.63                            |        | -0.42                          | 1.61                           | 0.83                            | -0.78  |
| GJ 905     | C      | 7.13                           | 2.33                           | 7.26                            | -0.06  |                                |                                | 7.68                            |        | 2.90                           | 1.71                           | 3.90                            | -0.58  |
| GJ 1002    | C      | 1.70                           | 2.88                           | 2.03                            | -0.11  |                                |                                | 2.14                            |        | 1.24                           | 1.68                           | 1.12                            | 0.07   |
| GJ 1057    | C      |                                |                                | 1.29                            |        |                                |                                | 1.36                            |        | 3.75                           | 1.64                           | 0.71                            | 1.85   |
| GJ 1093    | C      |                                |                                | 0.99                            |        |                                |                                | 1.05                            |        | 2.93                           | 1.69                           | 0.55                            | 1.41   |
| GJ 1111    | C      | -1.35                          | 2.76                           | 2.54                            | -1.41  |                                |                                | 2.69                            |        | -2.58                          | 1.56                           | 1.42                            | -2.57  |
| GJ 1151    | C      |                                |                                | 1.58                            |        |                                |                                | 1.67                            |        | -1.33                          | 1.68                           | 0.85                            | -1.30  |
| GJ 1156    | C      |                                |                                | 1.78                            |        |                                |                                | 1.88                            |        | 2.66                           | 1.64                           | 0.98                            | 1.03   |
| GJ 1214    | P      |                                |                                | 0.48                            |        |                                |                                | 0.51                            |        | 0.95                           | 1.06                           | 0.26                            | 0.65   |
| GJ 1227    | C      |                                |                                | 1.45                            |        |                                |                                | 1.53                            |        | 0.88                           | 1.67                           | 0.78                            | 0.06   |
| GJ 1286    | C      |                                |                                | 1.02                            |        |                                |                                | 1.08                            |        | 4.31                           | 1.64                           | 0.56                            | 2.29   |
| GJ 1289    | C      |                                |                                | 2.27                            |        |                                |                                | 2.40                            |        | 1.12                           | 1.77                           | 1.23                            | -0.06  |
| GJ 2005    | C      |                                |                                | 1.27                            |        |                                |                                | 1.34                            |        | 1.81                           | 1.73                           | 0.70                            | 0.65   |

| Name       | Sample | MIPS 70 $\mu\text{m}$         |                                |                                |        | PACS 70 $\mu\text{m}$         |                                |                                |        | PACS 100 $\mu\text{m}$        |                                |                                |        |
|------------|--------|-------------------------------|--------------------------------|--------------------------------|--------|-------------------------------|--------------------------------|--------------------------------|--------|-------------------------------|--------------------------------|--------------------------------|--------|
|            |        | $F_{\nu,\text{obs}}$<br>/ mJy | $\sigma_{\text{obs}}$<br>/ mJy | $F_{\nu,\text{pred}}$<br>/ mJy | $\chi$ | $F_{\nu,\text{obs}}$<br>/ mJy | $\sigma_{\text{obs}}$<br>/ mJy | $F_{\nu,\text{pred}}$<br>/ mJy | $\chi$ | $F_{\nu,\text{obs}}$<br>/ mJy | $\sigma_{\text{obs}}$<br>/ mJy | $F_{\nu,\text{pred}}$<br>/ mJy | $\chi$ |
| GJ 3146    | C      |                               |                                | 0.53                           |        |                               |                                | 0.56                           |        | -3.80                         | 1.57                           | 0.29                           | -2.61  |
| GJ 3207    | C      |                               |                                | 0.41                           |        |                               |                                | 0.43                           |        | -2.16                         | 1.54                           | 0.22                           | -1.55  |
| GJ 3323    | P      |                               |                                | 3.51                           |        |                               |                                | 3.71                           |        | 2.94                          | 1.68                           | 1.91                           | 0.62   |
| GJ 3378    | C      |                               |                                | 3.73                           |        |                               |                                | 3.95                           |        | 4.60                          | 1.73                           | 2.00                           | 1.50   |
| GJ 3454    | C      |                               |                                | 2.16                           |        |                               |                                | 2.28                           |        | 2.49                          | 1.46                           | 1.16                           | 0.90   |
| GJ 3522    | C      |                               |                                | 8.42                           |        |                               |                                | 8.90                           |        | 1.62                          | 1.62                           | 4.45                           | -1.75  |
| GJ 3622    | C      | 1.82                          | 1.96                           | 1.38                           | 0.23   |                               |                                | 1.46                           |        | -5.19                         | 1.61                           | 0.77                           | -3.70  |
| GJ 3634    | P      |                               |                                | 1.39                           |        |                               |                                | 1.47                           |        | -0.90                         | 1.21                           | 0.73                           | -1.35  |
| GJ 3737    | C      |                               |                                | 2.06                           |        |                               |                                | 2.17                           |        | 3.27                          | 1.61                           | 1.11                           | 1.33   |
| GJ 3877    | C      |                               |                                | 0.72                           |        |                               |                                | 0.76                           |        | -2.63                         | 1.56                           | 0.40                           | -1.94  |
| GJ 3959    | C      |                               |                                | 0.67                           |        |                               |                                | 0.71                           |        | 3.30                          | 1.68                           | 0.36                           | 1.74   |
| GJ 4053    | C      |                               |                                | 1.21                           |        |                               |                                | 1.28                           |        | -2.87                         | 1.72                           | 0.66                           | -2.06  |
| GJ 4063    | C      |                               |                                | 4.61                           |        |                               |                                | 4.87                           |        | 6.48                          | 1.72                           | 2.43                           | 2.36   |
| GJ 4248    | C      |                               |                                | 3.31                           |        |                               |                                | 3.49                           |        | 3.76                          | 1.68                           | 1.74                           | 1.19   |
| GJ 4274    | C      |                               |                                | 2.21                           |        |                               |                                | 2.34                           |        | 8.10                          | 2.04                           | 1.20                           | 3.38   |
| BD-10 3166 | P      | -4.46                         | 3.17                           | 0.44                           | -1.55  |                               |                                | 0.46                           |        |                               |                                | 0.23                           |        |
| LHS 22     | C      |                               |                                | 1.27                           |        |                               |                                | 1.35                           |        | 1.51                          | 1.70                           | 0.70                           | 0.47   |
| LHS 60     | C      |                               |                                | 2.98                           |        |                               |                                | 3.15                           |        | 4.58                          | 1.62                           | 1.59                           | 1.85   |
| LHS 1565   | C      | -2.10                         | 1.97                           | 4.17                           | -3.19  |                               |                                | 4.41                           |        | -0.66                         | 1.59                           | 2.31                           | -1.88  |
| LHS 1989   | C      |                               |                                | 3.51                           |        |                               |                                | 3.71                           |        | -3.93                         | 1.87                           | 1.88                           | -3.10  |
| LHS 2090   | C      |                               |                                | 0.83                           |        |                               |                                | 0.88                           |        | -2.04                         | 1.41                           | 0.46                           | -1.78  |
| PLX 2890   | C      | 3.96                          | 2.71                           | 6.84                           | -1.06  |                               |                                | 7.23                           |        | 4.36                          | 1.71                           | 3.78                           | 0.34   |
| PLX 4459   | C      |                               |                                | 3.94                           |        |                               |                                | 4.16                           |        | 0.02                          | 1.45                           | 2.07                           | -1.41  |
