# Supplementary material for: No significant correlation between radial velocity planet presence and debris disc properties
Source: arXiv:2005.03573 ancillary file (2020-05-07)
Supplement: Supplementary file 4 [file table4.pdf]

Full version of Table 4

| Name      | Sample | $T / \text{K}$ | $\sigma_T / \text{K}$ | $f$     | $\sigma_f$ |
|-----------|--------|----------------|-----------------------|---------|------------|
| HD 166    | C      | 79             | 2                     | 4.9E-05 | 1.4E-06    |
| HD 1461   | P      | 57             | 1                     | 4.3E-05 | 1.5E-06    |
| HD 5133   | C      | 62             | 4                     | 1.1E-05 | 1.1E-06    |
| HD 10647  | P      | 40             | 1                     | 2.4E-04 | 8.8E-06    |
| HD 10700  | P      | 104            | 9                     | 1.5E-05 | 2.8E-06    |
| HD 16673  | C      | 94             | 11                    | 5.9E-06 | 5.5E-07    |
| HD 17925  | C      | 81             | 10                    | 3.5E-05 | 6.1E-06    |
| HD 22049  | P      | 51             | 11                    | 4.2E-05 | 2.2E-05    |
| HD 22484  | C      | 88             | 6                     | 9.4E-06 | 7.7E-07    |
| HD 23356  | C      | 61             | 3                     | 1.7E-05 | 1.4E-06    |
| HD 30495  | C      | 61             | 6                     | 3.3E-05 | 1.8E-06    |
| HD 33262  | C      | 120            | 36                    | 1.6E-05 | 3.3E-06    |
| HD 38529  | P      | 44             | 9                     | 2.6E-05 | 2.6E-06    |
| HD 45184  | P      | 50             | 2                     | 7.0E-05 | 2.9E-06    |
| HD 48682  | C      | 51             | 1                     | 5.5E-05 | 9.5E-07    |
| HD 50499  | P      | 26             | 5                     | 1.3E-05 | 1.6E-06    |
| HD 50554  | P      | 53             | 6                     | 4.0E-05 | 1.3E-06    |
| HD 52265  | P      | 60             | 2                     | 1.8E-05 | 1.2E-06    |
| HD 72659  | P      | 40             | 10                    | 1.3E-05 | 2.6E-06    |
| HD 72905  | C      | 89             | 7                     | 8.2E-06 | 9.5E-07    |
| HD 76151  | C      | 101            | 8                     | 1.4E-05 | 9.4E-07    |
| HD 82943  | P      | 47             | 2                     | 9.5E-05 | 3.5E-06    |
| HD 90089  | C      | 32             | 1                     | 1.0E-05 | 5.3E-07    |
| HD 104067 | P      | 41             | 3                     | 8.8E-05 | 2.1E-05    |
| HD 106252 | P      | 40             | 13                    | 8.2E-06 | 2.2E-06    |
| HD 110897 | C      | 50             | 4                     | 2.2E-05 | 1.3E-06    |
| HD 113337 | P      | 54             | 1                     | 9.2E-05 | 2.6E-06    |
| HD 115617 | P      | 59             | 2                     | 2.3E-05 | 1.2E-06    |
| HD 117043 | C      | 78             | 8                     | 7.7E-06 | 9.3E-07    |
| HD 117176 | P      | 23             | 5                     | 2.6E-06 | 3.2E-07    |
| HD 128165 | C      | 58             | 8                     | 6.9E-06 | 9.6E-07    |
| HD 128311 | P      | 33             | 8                     | 2.5E-05 | 2.1E-06    |
| HD 150706 | P      | 61             | 6                     | 5.6E-05 | 8.0E-06    |
| HD 154577 | C      | 53             | 10                    | 1.5E-05 | 2.4E-06    |
| HD 158633 | C      | 57             | 2                     | 2.5E-05 | 1.2E-06    |
| HD 160032 | C      | 78             | 4                     | 5.4E-06 | 4.2E-07    |
| HD 169830 | P      | 32             | 11                    | 2.0E-06 | 5.6E-07    |
| HD 187085 | P      | 47             | 7                     | 1.6E-05 | 2.8E-06    |
| HD 192263 | P      | 57             | 11                    | 4.9E-05 | 7.6E-06    |
| HD 199260 | C      | 72             | 4                     | 1.5E-05 | 6.6E-07    |
| HD 202206 | P      | 55             | 1                     | 1.2E-04 | 3.3E-06    |
| HD 207129 | C      | 39             | 2                     | 8.8E-05 | 3.3E-06    |
| HD 216435 | P      | 46             | 10                    | 1.9E-05 | 1.7E-06    |
| HD 218511 | C      | 21             | 5                     | 1.6E-05 | 4.5E-06    |
| HD 219482 | C      | 86             | 3                     | 2.7E-05 | 7.1E-07    |
| HD 222368 | C      | 98             | 15                    | 2.9E-06 | 7.2E-07    |
| HIP 1368  | C      | 25             | 6                     | 9.4E-05 | 9.4E-06    |
| HIP 56528 | P      | 31             | 11                    | 2.6E-05 | 6.8E-06    |

| Name      | Sample | $T / \text{K}$ | $\sigma_T / \text{K}$ | $f$     | $\sigma_f$ |
|-----------|--------|----------------|-----------------------|---------|------------|
| HIP 74995 | P      | 48             | 8                     | 5.0E-05 | 5.6E-06    |
| HIP 83043 | P      | 44             | 14                    | 6.0E-05 | 1.9E-05    |
| HIP 88745 | C      | 45             | 4                     | 1.6E-05 | 9.9E-07    |
