# Supplementary material for: No significant correlation between radial velocity planet presence and debris disc properties
Source: arXiv:2005.03573 ancillary file (2020-05-07)
Supplement: Supplementary file 5 [file table5.pdf]

## Full version of Table 5

| Name     | Sample | $f_{\text{lim}}$ |
|----------|--------|------------------|
| HD 142   | P      | 2.4E-06          |
| HD 693   | C      | 1.7E-06          |
| HD 739   | C      | 2.3E-06          |
| HD 1237  | P      | 6.3E-06          |
| HD 1326  | P      | 1.1E-05          |
| HD 1581  | C      | 1.2E-06          |
| HD 1835  | C      | 6.1E-06          |
| HD 3443  | C      | 2.3E-06          |
| HD 3651  | P      | 2.7E-06          |
| HD 4203  | P      | 1.0E-04          |
| HD 4208  | P      | 4.5E-05          |
| HD 4308  | P      | 4.2E-06          |
| HD 4391  | C      | 3.5E-06          |
| HD 4628  | C      | 3.1E-06          |
| HD 4676  | C      | 1.9E-06          |
| HD 4747  | C      | 1.1E-05          |
| HD 4813  | C      | 1.6E-06          |
| HD 4967  | C      | 3.2E-05          |
| HD 6434  | P      | 6.7E-05          |
| HD 7439  | C      | 2.5E-06          |
| HD 7570  | C      | 1.9E-06          |
| HD 7924  | P      | 1.1E-05          |
| HD 8574  | P      | 8.8E-06          |
| HD 8673  | P      | 4.0E-06          |
| HD 9540  | C      | 9.8E-06          |
| HD 9826  | P      | 1.0E-06          |
| HD 10307 | C      | 1.7E-06          |
| HD 10361 | C      | 5.5E-06          |
| HD 10476 | C      | 2.1E-06          |
| HD 10697 | P      | 5.0E-06          |
| HD 11507 | C      | 9.8E-06          |
| HD 11964 | P      | 3.5E-06          |
| HD 12661 | P      | 1.1E-05          |
| HD 13445 | P      | 2.8E-06          |
| HD 13974 | C      | 1.7E-06          |
| HD 14412 | C      | 2.6E-06          |
| HD 16141 | P      | 5.6E-06          |
| HD 16160 | C      | 2.6E-06          |
| HD 16175 | P      | 9.7E-06          |
| HD 16417 | P      | 2.1E-06          |
| HD 16765 | C      | 4.2E-06          |
| HD 17051 | P      | 2.6E-06          |
| HD 17206 | C      | 1.2E-06          |
| HD 19305 | C      | 2.8E-05          |
| HD 20010 | C      | 1.1E-06          |
| HD 20630 | C      | 1.8E-06          |
| HD 20782 | P      | 1.1E-05          |
| HD 20794 | P      | 1.3E-06          |

| Name     | Sample | $f_{\text{lim}}$ |
|----------|--------|------------------|
| HD 20807 | C      | 1.6E-06          |
| HD 21197 | C      | 1.8E-05          |
| HD 21411 | P      | 7.3E-05          |
| HD 21531 | C      | 8.8E-06          |
| HD 22496 | C      | 2.2E-05          |
| HD 23079 | P      | 8.4E-06          |
| HD 23127 | P      | 9.8E-05          |
| HD 23596 | P      | 1.1E-05          |
| HD 23754 | C      | 1.1E-06          |
| HD 26965 | P      | 1.3E-06          |
| HD 27274 | C      | 6.0E-06          |
| HD 27894 | P      | 1.5E-04          |
| HD 28185 | P      | 3.3E-05          |
| HD 30177 | P      | 8.3E-05          |
| HD 30562 | P      | 2.3E-06          |
| HD 30652 | C      | 7.3E-07          |
| HD 32147 | C      | 3.6E-06          |
| HD 33283 | P      | 7.0E-05          |
| HD 33564 | P      | 2.0E-06          |
| HD 33793 | P      | 1.8E-05          |
| HD 34445 | P      | 2.8E-05          |
| HD 36435 | C      | 1.0E-05          |
| HD 36705 | C      | 8.2E-06          |
| HD 37124 | P      | 1.7E-05          |
| HD 37605 | P      | 2.0E-04          |
| HD 38393 | C      | 1.3E-06          |
| HD 39091 | P      | 3.4E-06          |
| HD 39855 | P      | 7.9E-05          |
| HD 40307 | P      | 5.0E-06          |
| HD 40979 | P      | 7.3E-06          |
| HD 41004 | P      | 2.8E-05          |
| HD 42581 | P      | 1.2E-05          |
| HD 43162 | C      | 2.9E-06          |
| HD 43834 | C      | 1.8E-06          |
| HD 45350 | P      | 6.1E-05          |
| HD 46588 | C      | 1.7E-06          |
| HD 49674 | P      | 6.4E-05          |
| HD 50692 | C      | 1.9E-06          |
| HD 52711 | C      | 2.2E-06          |
| HD 53705 | C      | 5.6E-06          |
| HD 55575 | C      | 2.0E-06          |
| HD 58855 | C      | 1.5E-06          |
| HD 60532 | P      | 1.5E-06          |
| HD 61606 | C      | 1.1E-05          |
| HD 62613 | C      | 3.1E-06          |
| HD 63454 | P      | 1.4E-04          |
| HD 65216 | P      | 5.1E-05          |
| HD 66428 | P      | 7.6E-05          |
| HD 68146 | C      | 5.1E-06          |
| HD 68988 | P      | 6.2E-05          |
| HD 69830 | P      | 2.3E-06          |
| HD 69897 | C      | 2.9E-06          |
| HD 70573 | P      | 1.3E-04          |
| HD 71243 | C      | 1.1E-06          |
| HD 73526 | P      | 5.0E-04          |
| HD 74156 | P      | 4.9E-05          |
| HD 75289 | P      | 9.3E-05          |

| Name      | Sample | $f_{\text{lim}}$ |
|-----------|--------|------------------|
| HD 75732  | P      | 3.5E-06          |
| HD 76700  | P      | 6.2E-05          |
| HD 76932  | C      | 3.6E-06          |
| HD 76943  | C      | 8.4E-07          |
| HD 78154  | C      | 2.2E-06          |
| HD 78366  | C      | 2.1E-06          |
| HD 79028  | C      | 1.8E-06          |
| HD 79096  | C      | 7.7E-06          |
| HD 79210  | C      | 8.9E-06          |
| HD 80606  | P      | 1.6E-04          |
| HD 81040  | P      | 4.8E-05          |
| HD 81997  | C      | 1.9E-06          |
| HD 82106  | C      | 5.0E-06          |
| HD 82328  | C      | 8.2E-07          |
| HD 83443  | P      | 7.8E-05          |
| HD 84117  | C      | 1.7E-06          |
| HD 84737  | C      | 1.8E-06          |
| HD 85512  | P      | 6.3E-06          |
| HD 86728  | C      | 2.0E-06          |
| HD 87883  | P      | 1.0E-05          |
| HD 88133  | P      | 6.3E-05          |
| HD 88230  | C      | 2.6E-06          |
| HD 89125  | C      | 4.6E-06          |
| HD 89269  | C      | 7.0E-06          |
| HD 89307  | P      | 6.3E-06          |
| HD 89449  | C      | 1.6E-06          |
| HD 89744  | P      | 2.1E-06          |
| HD 90156  | P      | 4.1E-05          |
| HD 90839  | C      | 1.7E-06          |
| HD 92788  | P      | 1.1E-05          |
| HD 93083  | P      | 6.9E-05          |
| HD 95128  | P      | 1.7E-06          |
| HD 95735  | P      | 5.3E-06          |
| HD 97101  | C      | 9.4E-06          |
| HD 97584  | C      | 1.4E-05          |
| HD 97658  | P      | 6.5E-05          |
| HD 98712  | C      | 2.5E-05          |
| HD 99492  | P      | 1.4E-05          |
| HD 100180 | C      | 5.5E-06          |
| HD 100623 | C      | 3.1E-06          |
| HD 101177 | C      | 5.5E-06          |
| HD 101501 | C      | 2.1E-06          |
| HD 101581 | C      | 1.3E-05          |
| HD 101930 | P      | 1.3E-04          |
| HD 102117 | P      | 2.7E-05          |
| HD 102195 | P      | 7.2E-05          |
| HD 102365 | P      | 1.9E-06          |
| HD 102438 | C      | 3.0E-06          |
| HD 102870 | C      | 9.5E-07          |
| HD 103095 | C      | 2.9E-06          |
| HD 103932 | C      | 3.7E-06          |
| HD 106516 | C      | 5.0E-06          |
| HD 107148 | P      | 7.2E-05          |
| HD 108147 | P      | 1.9E-04          |
| HD 108874 | P      | 1.1E-04          |
| HD 108954 | C      | 5.2E-06          |
| HD 109358 | C      | 1.0E-06          |

| Name      | Sample | $f_{\text{lim}}$ |
|-----------|--------|------------------|
| HD 109749 | P      | 7.0E-05          |
| HD 110315 | C      | 1.4E-05          |
| HD 110833 | C      | 4.3E-06          |
| HD 111232 | P      | 1.8E-05          |
| HD 111395 | C      | 2.3E-06          |
| HD 111631 | C      | 1.6E-05          |
| HD 113538 | P      | 3.7E-05          |
| HD 114386 | P      | 8.0E-05          |
| HD 114613 | P      | 5.9E-06          |
| HD 114710 | C      | 9.4E-07          |
| HD 114729 | P      | 5.5E-06          |
| HD 114762 | P      | 8.3E-06          |
| HD 114783 | P      | 9.8E-06          |
| HD 115404 | C      | 3.6E-06          |
| HD 116442 | C      | 1.1E-05          |
| HD 117207 | P      | 8.4E-06          |
| HD 117618 | P      | 9.7E-06          |
| HD 118203 | P      | 6.1E-05          |
| HD 118926 | C      | 4.9E-05          |
| HD 119850 | C      | 1.2E-05          |
| HD 120036 | C      | 2.6E-05          |
| HD 120136 | P      | 2.7E-06          |
| HD 120467 | C      | 1.8E-05          |
| HD 120476 | C      | 5.1E-06          |
| HD 120690 | C      | 3.1E-06          |
| HD 121504 | P      | 1.6E-04          |
| HD 122064 | C      | 2.7E-06          |
| HD 122742 | C      | 2.5E-06          |
| HD 124580 | C      | 5.5E-06          |
| HD 125276 | C      | 3.0E-06          |
| HD 126053 | C      | 2.3E-06          |
| HD 126660 | C      | 1.3E-06          |
| HD 128642 | C      | 4.5E-06          |
| HD 129502 | C      | 9.2E-07          |
| HD 130322 | P      | 1.0E-04          |
| HD 130948 | C      | 1.8E-06          |
| HD 131156 | C      | 3.1E-06          |
| HD 131511 | C      | 6.7E-06          |
| HD 131977 | C      | 3.3E-06          |
| HD 134083 | C      | 1.4E-06          |
| HD 134987 | P      | 3.5E-06          |
| HD 135204 | C      | 6.8E-06          |
| HD 136352 | P      | 4.3E-06          |
| HD 136923 | C      | 1.2E-05          |
| HD 137763 | C      | 1.2E-05          |
| HD 139763 | C      | 2.9E-05          |
| HD 140538 | C      | 2.9E-06          |
| HD 141004 | C      | 1.2E-06          |
| HD 141272 | C      | 1.4E-05          |
| HD 141937 | P      | 1.2E-05          |
| HD 142022 | P      | 1.4E-05          |
| HD 142267 | C      | 4.3E-06          |
| HD 142373 | C      | 1.3E-06          |
| HD 142415 | P      | 3.1E-05          |
| HD 142860 | C      | 8.3E-07          |
| HD 143105 | P      | 2.5E-05          |
| HD 143761 | P      | 1.7E-06          |

| Name       | Sample | $f_{\text{lim}}$ |
|------------|--------|------------------|
| HD 144579  | C      | 4.7E-06          |
| HD 145675  | P      | 3.9E-06          |
| HD 146361  | C      | 2.8E-06          |
| HD 147379  | P      | 1.9E-05          |
| HD 147513  | P      | 3.2E-06          |
| HD 147584  | C      | 1.5E-06          |
| HD 149026  | P      | 6.6E-05          |
| HD 149143  | P      | 5.9E-05          |
| HD 151288  | C      | 1.2E-05          |
| HD 153597  | C      | 1.0E-06          |
| HD 154345  | P      | 3.9E-06          |
| HD 154857  | P      | 1.0E-05          |
| HD 155358  | P      | 8.9E-06          |
| HD 155876  | C      | 7.0E-06          |
| HD 156668  | P      | 1.2E-04          |
| HD 156846  | P      | 5.7E-06          |
| HD 157214  | C      | 1.9E-06          |
| HD 157881  | C      | 6.8E-06          |
| HD 159868  | P      | 1.6E-05          |
| HD 160691  | P      | 1.9E-06          |
| HD 160922  | C      | 1.5E-06          |
| HD 162004  | P      | 4.1E-06          |
| HD 162020  | P      | 3.3E-04          |
| HD 164922  | P      | 6.7E-06          |
| HD 165499  | C      | 1.8E-06          |
| HD 166348  | C      | 2.2E-05          |
| HD 166620  | C      | 3.2E-06          |
| HD 167425  | C      | 5.3E-06          |
| HD 168151  | C      | 1.7E-06          |
| HD 168443  | P      | 2.0E-04          |
| HD 168746  | P      | 3.1E-03          |
| HD 170153  | C      | 8.1E-07          |
| HD 173739  | C      | 1.1E-05          |
| HD 177565  | P      | 1.3E-05          |
| HD 178911B | P      | 4.9E-05          |
| HD 179930  | C      | 3.3E-05          |
| HD 179949  | P      | 3.2E-06          |
| HD 180161  | C      | 1.0E-05          |
| HD 180617  | P      | 7.1E-05          |
| HD 181321  | C      | 7.3E-06          |
| HD 183263  | P      | 9.5E-05          |
| HD 185269  | P      | 6.0E-06          |
| HD 185395  | C      | 1.4E-06          |
| HD 186427  | P      | 6.3E-06          |
| HD 187123  | P      | 7.5E-05          |
| HD 188015  | P      | 2.7E-04          |
| HD 189245  | C      | 3.1E-06          |
| HD 189567  | C      | 2.4E-06          |
| HD 189733  | P      | 1.9E-05          |
| HD 190007  | C      | 1.0E-05          |
| HD 190422  | C      | 5.4E-06          |
| HD 191849  | C      | 9.4E-06          |
| HD 192310  | P      | 2.8E-06          |
| HD 194640  | C      | 7.1E-06          |
| HD 195019  | P      | 6.9E-06          |
| HD 196050  | P      | 2.5E-05          |
| HD 196761  | C      | 3.0E-06          |

| Name      | Sample | $f_{\text{lim}}$ |
|-----------|--------|------------------|
| HD 196877 | C      | 2.0E-05          |
| HD 196885 | P      | 4.4E-06          |
| HD 197076 | C      | 9.1E-06          |
| HD 197692 | C      | 1.0E-06          |
| HD 200525 | C      | 3.3E-06          |
| HD 200779 | C      | 1.9E-05          |
| HD 200968 | C      | 1.5E-05          |
| HD 202275 | C      | 1.3E-06          |
| HD 202560 | C      | 4.6E-06          |
| HD 203244 | C      | 9.2E-06          |
| HD 203608 | C      | 1.2E-06          |
| HD 204961 | P      | 1.1E-05          |
| HD 205390 | C      | 4.8E-06          |
| HD 208487 | P      | 4.0E-05          |
| HD 209100 | C      | 1.6E-06          |
| HD 209458 | P      | 4.9E-05          |
| HD 210027 | C      | 7.7E-07          |
| HD 210277 | P      | 4.0E-06          |
| HD 210302 | C      | 1.5E-06          |
| HD 211970 | P      | 2.7E-05          |
| HD 212301 | P      | 4.9E-05          |
| HD 212330 | C      | 2.2E-06          |
| HD 213240 | P      | 6.4E-06          |
| HD 213845 | C      | 2.3E-06          |
| HD 214749 | C      | 1.3E-05          |
| HD 214953 | C      | 5.4E-06          |
| HD 215152 | P      | 1.0E-04          |
| HD 215648 | C      | 1.1E-06          |
| HD 216133 | C      | 4.5E-05          |
| HD 216437 | P      | 2.7E-06          |
| HD 216770 | P      | 6.5E-05          |
| HD 216899 | C      | 1.2E-05          |
| HD 217014 | P      | 5.0E-06          |
| HD 217107 | P      | 4.6E-06          |
| HD 217357 | C      | 6.6E-06          |
| HD 217987 | C      | 5.5E-06          |
| HD 219134 | P      | 1.4E-05          |
| HD 219571 | C      | 1.0E-06          |
| HD 221420 | P      | 7.9E-06          |
| HD 221503 | C      | 2.4E-05          |
| HD 222237 | C      | 4.1E-06          |
| HD 222335 | C      | 1.1E-05          |
| HD 222582 | P      | 3.4E-05          |
| HD 224693 | P      | 7.0E-05          |
| HD 224953 | C      | 6.0E-05          |
| HD 225213 | C      | 1.1E-05          |
| HD 234078 | C      | 2.4E-05          |
| HD 265866 | C      | 2.3E-05          |
| HD 285968 | P      | 3.3E-05          |
| HD 330075 | P      | 7.5E-04          |
| HIP 171   | C      | 2.0E-06          |
| HIP 1242  | C      | 7.1E-05          |
| HIP 2762  | C      | 2.4E-06          |
| HIP 5496  | C      | 2.0E-05          |
| HIP 5643  | P      | 8.3E-05          |
| HIP 12961 | P      | 2.5E-04          |
| HIP 13375 | C      | 4.7E-05          |

| Name      | Sample | $f_{\text{lim}}$ |
|-----------|--------|------------------|
| HIP 14810 | P      | 1.0E-04          |
| HIP 18280 | C      | 3.2E-05          |
| HIP 19165 | P      | 2.1E-04          |
| HIP 22627 | P      | 8.8E-05          |
| HIP 23452 | C      | 1.2E-05          |
| HIP 27188 | C      | 2.6E-05          |
| HIP 31634 | C      | 4.1E-05          |
| HIP 33499 | C      | 5.3E-05          |
| HIP 34603 | C      | 4.4E-05          |
| HIP 36208 | P      | 1.9E-05          |
| HIP 37279 | C      | 6.1E-07          |
| HIP 37288 | C      | 3.6E-05          |
| HIP 37766 | C      | 4.8E-05          |
| HIP 38382 | C      | 1.9E-06          |
| HIP 38956 | C      | 1.1E-04          |
| HIP 42220 | C      | 3.0E-05          |
| HIP 42748 | C      | 4.0E-05          |
| HIP 43790 | P      | 2.3E-04          |
| HIP 43820 | C      | 1.4E-05          |
| HIP 44722 | C      | 3.0E-05          |
| HIP 47080 | C      | 2.4E-06          |
| HIP 49986 | C      | 1.8E-05          |
| HIP 51317 | C      | 2.6E-05          |
| HIP 52600 | C      | 2.7E-05          |
| HIP 53020 | C      | 6.5E-05          |
| HIP 53767 | C      | 2.6E-05          |
| HIP 54211 | C      | 1.8E-05          |
| HIP 55203 | C      | 1.0E-06          |
| HIP 57050 | P      | 6.1E-05          |
| HIP 57087 | P      | 3.4E-05          |
| HIP 57544 | C      | 5.2E-05          |
| HIP 57548 | P      | 4.5E-05          |
| HIP 61094 | C      | 3.5E-05          |
| HIP 61874 | C      | 1.9E-04          |
| HIP 62452 | C      | 7.0E-05          |
| HIP 63366 | C      | 1.7E-05          |
| HIP 64241 | C      | 1.1E-06          |
| HIP 65859 | C      | 2.0E-05          |
| HIP 66459 | C      | 2.1E-05          |
| HIP 67090 | C      | 4.4E-05          |
| HIP 70218 | C      | 2.1E-05          |
| HIP 70849 | P      | 7.4E-05          |
| HIP 70890 | P      | 3.2E-04          |
| HIP 71253 | C      | 4.4E-05          |
| HIP 73470 | C      | 2.4E-05          |
| HIP 73695 | C      | 1.9E-06          |
| HIP 76074 | C      | 1.7E-05          |
| HIP 80346 | C      | 3.9E-05          |
| HIP 80459 | P      | 4.0E-05          |
| HIP 80824 | P      | 7.0E-05          |
| HIP 83945 | C      | 8.6E-05          |
| HIP 85523 | P      | 2.5E-05          |
| HIP 85647 | P      | 2.4E-05          |
| HIP 86162 | P      | 1.2E-05          |
| HIP 86214 | P      | 3.1E-04          |
| HIP 86287 | P      | 2.9E-05          |
| HIP 86990 | C      | 4.6E-05          |

| Name       | Sample | $f_{\text{lim}}$ |
|------------|--------|------------------|
| HIP 93017  | C      | 2.1E-06          |
| HIP 99461  | C      | 2.1E-06          |
| HIP 103039 | C      | 5.8E-05          |
| HIP 105312 | C      | 3.7E-06          |
| HIP 106106 | C      | 2.8E-05          |
| HIP 106255 | C      | 7.6E-05          |
| HIP 107310 | C      | 1.4E-06          |
| HIP 109388 | P      | 2.5E-05          |
| HIP 110109 | C      | 2.0E-06          |
| HIP 110778 | C      | 2.9E-06          |
| HIP 113020 | P      | 2.1E-05          |
| HIP 117473 | C      | 1.8E-05          |
| GJ 55.3    | C      | 2.1E-06          |
| GJ 83.1    | C      | 9.9E-05          |
| GJ 299     | C      | 2.2E-04          |
| GJ 317     | P      | 8.6E-05          |
| GJ 388     | C      | 1.5E-05          |
| GJ 406     | C      | 1.0E-04          |
| GJ 493.1   | C      | 2.4E-04          |
| GJ 905     | C      | 5.5E-05          |
| GJ 1002    | C      | 2.2E-04          |
| GJ 1057    | C      | 3.2E-04          |
| GJ 1093    | C      | 4.8E-04          |
| GJ 1111    | C      | 2.0E-04          |
| GJ 1151    | C      | 2.3E-04          |
| GJ 1156    | C      | 2.4E-04          |
| GJ 1214    | P      | 4.7E-04          |
| GJ 1227    | C      | 2.7E-04          |
| GJ 1286    | C      | 4.4E-04          |
| GJ 1289    | C      | 1.7E-04          |
| GJ 2005    | C      | 4.7E-04          |
| GJ 3146    | C      | 8.8E-04          |
| GJ 3207    | C      | 6.8E-04          |
| GJ 3323    | P      | 1.0E-04          |
| GJ 3378    | C      | 9.3E-05          |
| GJ 3454    | C      | 1.6E-04          |
| GJ 3522    | C      | 3.7E-05          |
| GJ 3622    | C      | 3.8E-04          |
| GJ 3634    | P      | 1.3E-04          |
| GJ 3737    | C      | 1.7E-04          |
| GJ 3877    | C      | 8.1E-04          |
| GJ 3959    | C      | 5.8E-04          |
| GJ 4053    | C      | 3.2E-04          |
| GJ 4063    | C      | 6.9E-05          |
| GJ 4248    | C      | 9.5E-05          |
| GJ 4274    | C      | 2.2E-04          |
| BD-10 3166 | P      | 4.0E-04          |
| LHS 22     | C      | 3.3E-04          |
| LHS 60     | C      | 1.2E-04          |
| LHS 1565   | C      | 1.0E-04          |
| LHS 1989   | C      | 1.1E-04          |
| LHS 2090   | C      | 5.1E-04          |
| PLX 2890   | C      | 6.5E-05          |
| PLX 4459   | C      | 5.6E-05          |
