# Supplementary material for: No significant correlation between radial velocity planet presence and debris disc properties
Source: arXiv:2005.03573 ancillary file (2020-05-07)
Supplement: Supplementary file 6 [file table7.pdf]

Full version of Table 7

| Name     | Sample | $\Delta v_t / \text{ms}^{-1}$ | $M_{\text{anom}} / M_J$ | Known binary |
|----------|--------|-------------------------------|-------------------------|--------------|
| HD 142   | P      | 122.1                         | 12.5                    | Y            |
| HD 693   | C      | 574.1                         | 58.9                    | N            |
| HD 739   | C      | 708.5                         | 130.2                   | N            |
| HD 1326  | P      | 23.5                          | 2.7                     | Y            |
| HD 1581  | C      | 322.6                         | 29.6                    | N            |
| HD 4676  | C      | 56.4                          | 16.6                    | Y            |
| HD 4747  | C      | 301.2                         | 48.1                    | Y            |
| HD 8673  | P      | 98.3                          | 10.6                    | Y            |
| HD 9826  | P      | 93.1                          | 6.2                     | Y            |
| HD 10307 | C      | 774.9                         | 172.8                   | Y            |
| HD 10361 | C      | 182.7                         | 98.2                    | Y            |
| HD 10476 | C      | 39.7                          | 19.6                    | Y            |
| HD 10647 | P      | 9.9                           | 21.1                    | N            |
| HD 10697 | P      | 80.4                          | 8.0                     | Y            |
| HD 10700 | P      | 131.9                         | 10.6                    | Y            |
| HD 13445 | P      | 937.8                         | 96.1                    | Y            |
| HD 13974 | C      | 221.8                         | 19.5                    | Y            |
| HD 16141 | P      | 33.2                          | 44.2                    | Y            |
| HD 16160 | C      | 978.3                         | 72.5                    | Y            |
| HD 16765 | C      | 25.3                          | 72.6                    | Y            |
| HD 17051 | P      | 14.5                          | 11.7                    | N            |
| HD 17206 | C      | 1532.4                        | 157.1                   | N            |
| HD 20010 | C      | 359.4                         | 65.2                    | Y            |
| HD 20794 | P      | 111.0                         | 9.4                     | N            |
| HD 23596 | P      | 165.5                         | 17.2                    | Y            |
| HD 23754 | C      | 107.7                         | 14.6                    | N            |
| HD 27894 | P      | 128.6                         | 10.1                    | N            |
| HD 30652 | C      | 74.9                          | 4.4                     | N            |
| HD 33262 | C      | 10.8                          | 6.6                     | Y            |
| HD 36705 | C      | 2078.5                        | 167.4                   | Y            |
| HD 38393 | C      | 188.4                         | 19.3                    | Y            |
| HD 38529 | P      | 147.5                         | 16.8                    | Y            |
| HD 39091 | P      | 81.3                          | 13.3                    | N            |
| HD 41004 | P      | 1076.4                        | 86.4                    | Y            |
| HD 42581 | P      | 112.7                         | 6.6                     | Y            |
| HD 48682 | C      | 74.7                          | 15.1                    | N            |
| HD 50692 | C      | 20.0                          | 21.5                    | N            |
| HD 63454 | P      | 64.6                          | 4.8                     | N            |
| HD 66428 | P      | 198.2                         | 18.6                    | N            |
| HD 68146 | C      | 8.0                           | 17.8                    | Y            |
| HD 69897 | C      | 38.2                          | 13.6                    | N            |
| HD 71243 | C      | 193.0                         | 11.1                    | N            |
| HD 72659 | P      | 150.1                         | 15.0                    | N            |
| HD 74156 | P      | 111.0                         | 11.4                    | N            |
| HD 76151 | C      | 26.4                          | 15.5                    | N            |
| HD 76932 | C      | 63.3                          | 6.1                     | N            |
| HD 76943 | C      | 4297.7                        | 462.9                   | Y            |
| HD 78154 | C      | 67.6                          | 23.9                    | Y            |

| Name       | Sample | $\Delta v_r / \text{ms}^{-1}$ | $M_{\text{anom}} / M_J$ | Known binary |
|------------|--------|-------------------------------|-------------------------|--------------|
| HD 79028   | C      | 192.3                         | 19.7                    | Y            |
| HD 79210   | C      | 66.4                          | 4.2                     | Y            |
| HD 81040   | P      | 80.3                          | 7.2                     | N            |
| HD 81997   | C      | 2287.6                        | 397.9                   | Y            |
| HD 82328   | C      | 358.1                         | 41.9                    | Y            |
| HD 82943   | P      | 44.7                          | 28.1                    | N            |
| HD 86728   | C      | 3.0                           | 10.4                    | N            |
| HD 87883   | P      | 98.3                          | 7.7                     | N            |
| HD 90089   | C      | 2392.8                        | 257.7                   | N            |
| HD 92788   | P      | 71.3                          | 6.7                     | N            |
| HD 97584   | C      | 20.4                          | 1.5                     | Y            |
| HD 98712   | C      | 990.8                         | 65.7                    | Y            |
| HD 100623  | C      | 41.3                          | 3.3                     | Y            |
| HD 101177  | C      | 49.9                          | 4.5                     | Y            |
| HD 102365  | P      | 15.3                          | 4.4                     | Y            |
| HD 103095  | C      | 1.0                           | 5.2                     | N            |
| HD 106252  | P      | 131.9                         | 12.5                    | N            |
| HD 109358  | C      | 453.0                         | 41.5                    | N            |
| HD 110315  | C      | 425.3                         | 34.4                    | N            |
| HD 110833  | C      | 380.6                         | 46.6                    | Y            |
| HD 113337  | P      | 139.3                         | 30.0                    | Y            |
| HD 114710  | C      | 104.8                         | 4.1                     | N            |
| HD 114729  | P      | 82.4                          | 66.3                    | Y            |
| HD 114762  | P      | 869.8                         | 84.5                    | Y            |
| HD 115404  | C      | 117.5                         | 7.3                     | Y            |
| HD 120036  | C      | 111.9                         | 7.4                     | Y            |
| HD 120136  | P      | 778.9                         | 83.9                    | Y            |
| HD 120476  | C      | 721.9                         | 48.5                    | Y            |
| HD 120690  | C      | 1213.3                        | 412.1                   | Y            |
| HD 122742  | C      | 474.4                         | 57.4                    | Y            |
| HD 125276  | C      | 127.2                         | 11.5                    | Y            |
| HD 129502  | C      | 763.6                         | 89.9                    | N            |
| HD 131156  | C      | 574.7                         | 60.5                    | Y            |
| HD 131511  | C      | 408.6                         | 32.8                    | Y            |
| HD 131977  | C      | 55.9                          | 9.8                     | Y            |
| HD 136352  | P      | 60.4                          | 5.5                     | N            |
| HD 137763  | C      | 1582.5                        | 178.8                   | Y            |
| HD 140538  | C      | 279.3                         | 25.0                    | Y            |
| HD 141937  | P      | 548.7                         | 50.3                    | N            |
| HD 142022  | P      | 66.4                          | 5.9                     | Y            |
| HD 142860  | C      | 81.9                          | 5.6                     | N            |
| HD 143761  | P      | 18.4                          | 18.8                    | Y            |
| HD 145675  | P      | 134.1                         | 11.5                    | Y            |
| HD 146361  | C      | 74.9                          | 95.1                    | Y            |
| HD 147513  | P      | 20.9                          | 19.4                    | Y            |
| HD 147584  | C      | 116.3                         | 11.0                    | Y            |
| HD 160691  | P      | 34.9                          | 17.5                    | N            |
| HD 160922  | C      | 117.7                         | 14.3                    | Y            |
| HD 162004  | P      | 93.1                          | 9.5                     | Y            |
| HD 162020  | P      | 207.0                         | 15.4                    | Y            |
| HD 165499  | C      | 432.0                         | 108.5                   | N            |
| HD 168443  | P      | 160.3                         | 71.9                    | Y            |
| HD 173739  | C      | 50.8                          | 20.9                    | Y            |
| HD 178911B | P      | 315.1                         | 28.6                    | Y            |
| HD 181321  | C      | 2429.9                        | 227.1                   | N            |
| HD 185395  | C      | 148.1                         | 19.7                    | Y            |
| HD 186427  | P      | 29.5                          | 2.8                     | Y            |

| Name       | Sample | $\Delta v_t / \text{ms}^{-1}$ | $M_{\text{anom}} / M_J$ | Known binary |
|------------|--------|-------------------------------|-------------------------|--------------|
| HD 189245  | C      | 21.5                          | 28.8                    | N            |
| HD 196885  | P      | 1547.1                        | 313.9                   | Y            |
| HD 199260  | C      | 108.4                         | 10.5                    | N            |
| HD 200525  | C      | 3200.0                        | 540.4                   | Y            |
| HD 200968  | C      | 171.2                         | 13.7                    | Y            |
| HD 202275  | C      | 142.9                         | 29.5                    | Y            |
| HD 202560  | C      | 9.8                           | 0.6                     | N            |
| HD 203244  | C      | 4623.2                        | 392.5                   | N            |
| HD 204961  | P      | 12.5                          | 0.6                     | N            |
| HD 209100  | C      | 44.0                          | 3.2                     | Y            |
| HD 212330  | C      | 1284.3                        | 522.3                   | N            |
| HD 213240  | P      | 63.1                          | 6.4                     | Y            |
| HD 215648  | C      | 320.4                         | 34.8                    | Y            |
| HD 217014  | P      | 64.7                          | 6.1                     | Y            |
| HD 219482  | C      | 31.1                          | 19.3                    | N            |
| HD 219571  | C      | 2000.7                        | 247.5                   | N            |
| HD 221420  | P      | 217.2                         | 25.6                    | N            |
| HD 222237  | C      | 59.7                          | 4.4                     | N            |
| HD 222368  | C      | 190.6                         | 20.5                    | N            |
| HD 224953  | C      | 312.4                         | 19.7                    | Y            |
| HIP 171    | C      | 8233.0                        | 699.1                   | Y            |
| HIP 5496   | C      | 400.4                         | 22.6                    | N            |
| HIP 12961  | P      | 48.4                          | 3.1                     | N            |
| HIP 23452  | C      | 1575.8                        | 118.2                   | Y            |
| HIP 27188  | C      | 19.4                          | 1.3                     | N            |
| HIP 31634  | C      | 339.5                         | 21.9                    | Y            |
| HIP 33499  | C      | 575.3                         | 25.3                    | Y            |
| HIP 42220  | C      | 1483.3                        | 131.4                   | Y            |
| HIP 42748  | C      | 277.4                         | 17.9                    | Y            |
| HIP 47080  | C      | 92.7                          | 8.0                     | Y            |
| HIP 52600  | C      | 273.2                         | 17.6                    | Y            |
| HIP 63366  | C      | 358.3                         | 28.7                    | Y            |
| HIP 70849  | P      | 60.2                          | 3.9                     | N            |
| HIP 73470  | C      | 1351.2                        | 96.1                    | Y            |
| HIP 73695  | C      | 4785.6                        | 433.8                   | Y            |
| HIP 80346  | C      | 1640.3                        | 74.1                    | Y            |
| HIP 83945  | C      | 263.5                         | 9.7                     | Y            |
| HIP 85647  | P      | 120.0                         | 7.8                     | Y            |
| HIP 86162  | P      | 8.9                           | 0.4                     | N            |
| HIP 88745  | C      | 2311.6                        | 179.6                   | Y            |
| HIP 93017  | C      | 1869.3                        | 103.8                   | Y            |
| HIP 105312 | C      | 485.8                         | 20.5                    | Y            |
| HIP 106255 | C      | 1941.0                        | 73.9                    | Y            |
| HIP 107310 | C      | 246.6                         | 44.8                    | Y            |
| HIP 110109 | C      | 96.9                          | 15.4                    | Y            |
| HIP 110778 | C      | 9691.2                        | 834.0                   | Y            |
| GJ 55.3    | C      | 1636.0                        | 241.1                   | Y            |
